# Supplementary material for: Divisor Goldbach Conjecture and its Partition Number
Source: arXiv:1603.05233 source file (2016-03-14)
Supplement: Supplementary file 1 [file Appendix_III.pdf]

# Appendix III

| $n$ | $m$ | $q$ | $Y(m,n)$ |
|-----|-----|-----|----------|
| 4   | 2   | 2   | 1        |
| 6   | 2   | 3   | 1        |
| 6   | 3   | 2   | 1        |
| 8   | 2   | 4   | 1        |
| 8   | 4   | 2   | 1        |
| 9   | 3   | 3   | 2        |
| 10  | 2   | 5   | 2        |
| 10  | 5   | 2   | 1        |
| 12  | 2   | 6   | 1        |
| 12  | 3   | 4   | 2        |
| 12  | 4   | 3   | 2        |
| 12  | 6   | 2   | 1        |
| 14  | 2   | 7   | 2        |
| 14  | 7   | 2   | 1        |
| 15  | 3   | 5   | 3        |
| 15  | 5   | 3   | 3        |
| 16  | 2   | 8   | 2        |
| 16  | 4   | 4   | 3        |
| 16  | 8   | 2   | 1        |
| 18  | 2   | 9   | 2        |
| 18  | 3   | 6   | 2        |
| 18  | 6   | 3   | 4        |
| 18  | 9   | 2   | 1        |
| 20  | 2   | 10  | 2        |
| 20  | 4   | 5   | 6        |
| 20  | 5   | 4   | 4        |
| 20  | 10  | 2   | 1        |
| 21  | 3   | 7   | 5        |
| 21  | 7   | 3   | 4        |
| 22  | 2   | 11  | 3        |
| 22  | 11  | 2   | 1        |
| 24  | 2   | 12  | 3        |
| 24  | 3   | 8   | 3        |
| 24  | 4   | 6   | 7        |
| 24  | 6   | 4   | 8        |
| 24  | 8   | 3   | 5        |
| 24  | 12  | 2   | 1        |
| 25  | 5   | 5   | 10       |
| 26  | 2   | 13  | 3        |
| 26  | 13  | 2   | 1        |
| 27  | 3   | 9   | 7        |
| 27  | 9   | 3   | 7        |
| 28  | 2   | 14  | 2        |
| 28  | 4   | 7   | 11       |

|    |    |    |    |
|----|----|----|----|
| 28 | 7  | 4  | 10 |
| 28 | 14 | 2  | 1  |
| 30 | 2  | 15 | 3  |
| 30 | 3  | 10 | 2  |
| 30 | 5  | 6  | 11 |
| 30 | 6  | 5  | 16 |
| 30 | 10 | 3  | 8  |
| 30 | 15 | 2  | 1  |
| 32 | 2  | 16 | 2  |
| 32 | 4  | 8  | 13 |
| 32 | 8  | 4  | 16 |
| 32 | 16 | 2  | 1  |
| 33 | 3  | 11 | 9  |
| 33 | 11 | 3  | 10 |
| 34 | 2  | 17 | 4  |
| 34 | 17 | 2  | 1  |
| 35 | 5  | 7  | 20 |
| 35 | 7  | 5  | 26 |
| 36 | 2  | 18 | 4  |
| 36 | 3  | 12 | 4  |
| 36 | 4  | 9  | 15 |
| 36 | 6  | 6  | 26 |
| 36 | 9  | 4  | 21 |
| 36 | 12 | 3  | 12 |
| 36 | 18 | 2  | 1  |
| 38 | 2  | 19 | 2  |
| 38 | 19 | 2  | 1  |
| 39 | 3  | 13 | 10 |
| 39 | 13 | 3  | 13 |
| 40 | 2  | 20 | 3  |
| 40 | 4  | 10 | 21 |
| 40 | 5  | 8  | 18 |
| 40 | 8  | 5  | 39 |
| 40 | 10 | 4  | 31 |
| 40 | 20 | 2  | 1  |
| 42 | 2  | 21 | 4  |
| 42 | 3  | 14 | 3  |
| 42 | 6  | 7  | 42 |
| 42 | 7  | 6  | 33 |
| 42 | 14 | 3  | 16 |
| 42 | 21 | 2  | 1  |
| 44 | 2  | 22 | 3  |
| 44 | 4  | 11 | 24 |
| 44 | 11 | 4  | 38 |
| 44 | 22 | 2  | 1  |
| 45 | 3  | 15 | 12 |
| 45 | 5  | 9  | 38 |

|    |    |    |     |
|----|----|----|-----|
| 45 | 9  | 5  | 59  |
| 45 | 15 | 3  | 20  |
| 46 | 2  | 23 | 4   |
| 46 | 23 | 2  | 1   |
| 48 | 2  | 24 | 5   |
| 48 | 3  | 16 | 4   |
| 48 | 4  | 12 | 26  |
| 48 | 6  | 8  | 60  |
| 48 | 8  | 6  | 77  |
| 48 | 12 | 4  | 55  |
| 48 | 16 | 3  | 22  |
| 48 | 24 | 2  | 1   |
| 49 | 7  | 7  | 77  |
| 50 | 2  | 25 | 4   |
| 50 | 5  | 10 | 26  |
| 50 | 10 | 5  | 87  |
| 50 | 25 | 2  | 1   |
| 51 | 3  | 17 | 15  |
| 51 | 17 | 3  | 26  |
| 52 | 2  | 26 | 3   |
| 52 | 4  | 13 | 34  |
| 52 | 13 | 4  | 68  |
| 52 | 26 | 2  | 1   |
| 54 | 2  | 27 | 5   |
| 54 | 3  | 18 | 3   |
| 54 | 6  | 9  | 86  |
| 54 | 9  | 6  | 104 |
| 54 | 18 | 3  | 31  |
| 54 | 27 | 2  | 1   |
| 55 | 5  | 11 | 64  |
| 55 | 11 | 5  | 124 |
| 56 | 2  | 28 | 3   |
| 56 | 4  | 14 | 38  |
| 56 | 7  | 8  | 86  |
| 56 | 8  | 7  | 133 |
| 56 | 14 | 4  | 91  |
| 56 | 28 | 2  | 1   |
| 57 | 3  | 19 | 17  |
| 57 | 19 | 3  | 34  |
| 58 | 2  | 29 | 4   |
| 58 | 29 | 2  | 1   |
| 60 | 2  | 30 | 6   |
| 60 | 3  | 20 | 4   |
| 60 | 4  | 15 | 41  |
| 60 | 5  | 12 | 41  |
| 60 | 6  | 10 | 116 |
| 60 | 10 | 6  | 191 |

|    |    |    |     |
|----|----|----|-----|
| 60 | 12 | 5  | 178 |
| 60 | 15 | 4  | 116 |
| 60 | 20 | 3  | 41  |
| 60 | 30 | 2  | 1   |
| 62 | 2  | 31 | 3   |
| 62 | 31 | 2  | 1   |
| 63 | 3  | 21 | 19  |
| 63 | 7  | 9  | 174 |
| 63 | 9  | 7  | 236 |
| 63 | 21 | 3  | 48  |
| 64 | 2  | 32 | 5   |
| 64 | 4  | 16 | 50  |
| 64 | 8  | 8  | 227 |
| 64 | 16 | 4  | 153 |
| 64 | 32 | 2  | 1   |
| 65 | 5  | 13 | 92  |
| 65 | 13 | 5  | 248 |
| 66 | 2  | 33 | 6   |
| 66 | 3  | 22 | 5   |
| 66 | 6  | 11 | 156 |
| 66 | 11 | 6  | 261 |
| 66 | 22 | 3  | 53  |
| 66 | 33 | 2  | 1   |
| 68 | 2  | 34 | 2   |
| 68 | 4  | 17 | 56  |
| 68 | 17 | 4  | 182 |
| 68 | 34 | 2  | 1   |
| 69 | 3  | 23 | 20  |
| 69 | 23 | 3  | 61  |
| 70 | 2  | 35 | 5   |
| 70 | 5  | 14 | 56  |
| 70 | 7  | 10 | 171 |
| 70 | 10 | 7  | 396 |
| 70 | 14 | 5  | 345 |
| 70 | 35 | 2  | 1   |
| 72 | 2  | 36 | 6   |
| 72 | 3  | 24 | 5   |
| 72 | 4  | 18 | 57  |
| 72 | 6  | 12 | 202 |
| 72 | 8  | 9  | 360 |
| 72 | 9  | 8  | 318 |
| 72 | 12 | 6  | 457 |
| 72 | 18 | 4  | 242 |
| 72 | 24 | 3  | 70  |
| 72 | 36 | 2  | 1   |
| 74 | 2  | 37 | 5   |
| 74 | 37 | 2  | 1   |

|    |    |    |      |
|----|----|----|------|
| 75 | 3  | 25 | 22   |
| 75 | 5  | 15 | 140  |
| 75 | 15 | 5  | 471  |
| 75 | 25 | 3  | 78   |
| 76 | 2  | 38 | 5    |
| 76 | 4  | 19 | 70   |
| 76 | 19 | 4  | 292  |
| 76 | 38 | 2  | 1    |
| 77 | 7  | 11 | 359  |
| 77 | 11 | 7  | 638  |
| 78 | 2  | 39 | 7    |
| 78 | 3  | 26 | 5    |
| 78 | 6  | 13 | 259  |
| 78 | 13 | 6  | 601  |
| 78 | 26 | 3  | 90   |
| 78 | 39 | 2  | 1    |
| 80 | 2  | 40 | 4    |
| 80 | 4  | 20 | 77   |
| 80 | 5  | 16 | 67   |
| 80 | 8  | 10 | 533  |
| 80 | 10 | 8  | 729  |
| 80 | 16 | 5  | 637  |
| 80 | 20 | 4  | 369  |
| 80 | 40 | 2  | 1    |
| 81 | 3  | 27 | 25   |
| 81 | 9  | 9  | 683  |
| 81 | 27 | 3  | 103  |
| 82 | 2  | 41 | 5    |
| 82 | 41 | 2  | 1    |
| 84 | 2  | 42 | 8    |
| 84 | 3  | 28 | 5    |
| 84 | 4  | 21 | 81   |
| 84 | 6  | 14 | 323  |
| 84 | 7  | 12 | 295  |
| 84 | 12 | 7  | 1030 |
| 84 | 14 | 6  | 997  |
| 84 | 21 | 4  | 448  |
| 84 | 28 | 3  | 113  |
| 84 | 42 | 2  | 1    |
| 85 | 5  | 17 | 186  |
| 85 | 17 | 5  | 854  |
| 86 | 2  | 43 | 5    |
| 86 | 43 | 2  | 1    |
| 87 | 3  | 29 | 29   |
| 87 | 29 | 3  | 129  |
| 88 | 2  | 44 | 4    |
| 88 | 4  | 22 | 96   |

|     |    |    |      |
|-----|----|----|------|
| 88  | 8  | 11 | 789  |
| 88  | 11 | 8  | 1026 |
| 88  | 22 | 4  | 562  |
| 88  | 44 | 2  | 1    |
| 90  | 2  | 45 | 9    |
| 90  | 3  | 30 | 4    |
| 90  | 5  | 18 | 96   |
| 90  | 6  | 15 | 400  |
| 90  | 9  | 10 | 789  |
| 90  | 10 | 9  | 1259 |
| 90  | 15 | 6  | 1308 |
| 90  | 18 | 5  | 1134 |
| 90  | 30 | 3  | 147  |
| 90  | 45 | 2  | 1    |
| 91  | 7  | 13 | 656  |
| 91  | 13 | 7  | 1614 |
| 92  | 2  | 46 | 4    |
| 92  | 4  | 23 | 100  |
| 92  | 23 | 4  | 668  |
| 92  | 46 | 2  | 1    |
| 93  | 3  | 31 | 33   |
| 93  | 31 | 3  | 162  |
| 94  | 2  | 47 | 5    |
| 94  | 47 | 2  | 1    |
| 95  | 5  | 19 | 249  |
| 95  | 19 | 5  | 1494 |
| 96  | 2  | 48 | 7    |
| 96  | 3  | 32 | 5    |
| 96  | 4  | 24 | 109  |
| 96  | 6  | 16 | 489  |
| 96  | 8  | 12 | 1126 |
| 96  | 12 | 8  | 2101 |
| 96  | 16 | 6  | 2038 |
| 96  | 24 | 4  | 835  |
| 96  | 32 | 3  | 184  |
| 96  | 48 | 2  | 1    |
| 98  | 2  | 49 | 3    |
| 98  | 7  | 14 | 489  |
| 98  | 14 | 7  | 2464 |
| 98  | 49 | 2  | 1    |
| 99  | 3  | 33 | 30   |
| 99  | 9  | 11 | 1652 |
| 99  | 11 | 9  | 2286 |
| 99  | 33 | 3  | 206  |
| 100 | 2  | 50 | 6    |
| 100 | 4  | 25 | 126  |
| 100 | 5  | 20 | 114  |

|     |    |    |      |
|-----|----|----|------|
| 100 | 10 | 10 | 2104 |
| 100 | 20 | 5  | 1955 |
| 100 | 25 | 4  | 992  |
| 100 | 50 | 2  | 1    |
| 102 | 2  | 51 | 8    |
| 102 | 3  | 34 | 6    |
| 102 | 6  | 17 | 599  |
| 102 | 17 | 6  | 2671 |
| 102 | 34 | 3  | 226  |
| 102 | 51 | 2  | 1    |
| 104 | 2  | 52 | 5    |
| 104 | 4  | 26 | 129  |
| 104 | 8  | 13 | 1541 |
| 104 | 13 | 8  | 2912 |
| 104 | 26 | 4  | 1209 |
| 104 | 52 | 2  | 1    |
| 105 | 3  | 35 | 35   |
| 105 | 5  | 21 | 337  |
| 105 | 7  | 15 | 1092 |
| 105 | 15 | 7  | 3745 |
| 105 | 21 | 5  | 2534 |
| 105 | 35 | 3  | 256  |
| 106 | 2  | 53 | 6    |
| 106 | 53 | 2  | 1    |
| 108 | 2  | 54 | 8    |
| 108 | 3  | 36 | 6    |
| 108 | 4  | 27 | 138  |
| 108 | 6  | 18 | 713  |
| 108 | 9  | 12 | 1671 |
| 108 | 12 | 9  | 3986 |
| 108 | 18 | 6  | 4024 |
| 108 | 27 | 4  | 1438 |
| 108 | 36 | 3  | 286  |
| 108 | 54 | 2  | 1    |
| 110 | 2  | 55 | 6    |
| 110 | 5  | 22 | 138  |
| 110 | 10 | 11 | 3329 |
| 110 | 11 | 10 | 3028 |
| 110 | 22 | 5  | 3272 |
| 110 | 55 | 2  | 1    |
| 111 | 3  | 37 | 37   |
| 111 | 37 | 3  | 314  |
| 112 | 2  | 56 | 7    |
| 112 | 4  | 28 | 156  |
| 112 | 7  | 16 | 772  |
| 112 | 8  | 14 | 2103 |
| 112 | 14 | 8  | 5521 |

|     |    |    |      |
|-----|----|----|------|
| 112 | 16 | 7  | 5597 |
| 112 | 28 | 4  | 1749 |
| 112 | 56 | 2  | 1    |
| 114 | 2  | 57 | 10   |
| 114 | 3  | 38 | 7    |
| 114 | 6  | 19 | 853  |
| 114 | 19 | 6  | 5177 |
| 114 | 38 | 3  | 352  |
| 114 | 57 | 2  | 1    |
| 115 | 5  | 23 | 419  |
| 115 | 23 | 5  | 4188 |
| 116 | 2  | 58 | 6    |
| 116 | 4  | 29 | 163  |
| 116 | 29 | 4  | 2043 |
| 116 | 58 | 2  | 1    |
| 117 | 3  | 39 | 43   |
| 117 | 9  | 13 | 3501 |
| 117 | 13 | 9  | 6793 |
| 117 | 39 | 3  | 391  |
| 118 | 2  | 59 | 6    |
| 118 | 59 | 2  | 1    |
| 119 | 7  | 17 | 1738 |
| 119 | 17 | 7  | 8203 |
| 120 | 2  | 60 | 12   |
| 120 | 3  | 40 | 6    |
| 120 | 4  | 30 | 175  |
| 120 | 5  | 24 | 175  |
| 120 | 6  | 20 | 1003 |
| 120 | 8  | 15 | 2825 |
| 120 | 10 | 12 | 5089 |
| 120 | 12 | 10 | 7155 |
| 120 | 15 | 8  | 7600 |
| 120 | 20 | 6  | 7607 |
| 120 | 24 | 5  | 5343 |
| 120 | 30 | 4  | 2476 |
| 120 | 40 | 3  | 429  |
| 120 | 60 | 2  | 1    |
| 121 | 11 | 11 | 6480 |
| 122 | 2  | 61 | 4    |
| 122 | 61 | 2  | 1    |
| 123 | 3  | 41 | 47   |
| 123 | 41 | 3  | 479  |
| 124 | 2  | 62 | 5    |
| 124 | 4  | 31 | 199  |
| 124 | 31 | 4  | 2901 |
| 124 | 62 | 2  | 1    |
| 125 | 5  | 25 | 526  |

|     |    |    |       |
|-----|----|----|-------|
| 125 | 25 | 5  | 6768  |
| 126 | 2  | 63 | 10    |
| 126 | 3  | 42 | 5     |
| 126 | 6  | 21 | 1182  |
| 126 | 7  | 18 | 1120  |
| 126 | 9  | 14 | 3215  |
| 126 | 14 | 9  | 11411 |
| 126 | 18 | 7  | 11952 |
| 126 | 21 | 6  | 9721  |
| 126 | 42 | 3  | 530   |
| 126 | 63 | 2  | 1     |
| 128 | 2  | 64 | 3     |
| 128 | 4  | 32 | 198   |
| 128 | 8  | 16 | 3677  |
| 128 | 16 | 8  | 13547 |
| 128 | 32 | 4  | 3453  |
| 128 | 64 | 2  | 1     |
| 129 | 3  | 43 | 45    |
| 129 | 43 | 3  | 579   |
| 130 | 2  | 65 | 7     |
| 130 | 5  | 26 | 198   |
| 130 | 10 | 13 | 7648  |
| 130 | 13 | 10 | 10312 |
| 130 | 26 | 5  | 8537  |
| 130 | 65 | 2  | 1     |
| 132 | 2  | 66 | 9     |
| 132 | 3  | 44 | 7     |
| 132 | 4  | 33 | 211   |
| 132 | 6  | 22 | 1377  |
| 132 | 11 | 12 | 7648  |
| 132 | 12 | 11 | 12244 |
| 132 | 22 | 6  | 13840 |
| 132 | 33 | 4  | 4042  |
| 132 | 44 | 3  | 644   |
| 132 | 66 | 2  | 1     |
| 133 | 7  | 19 | 2686  |
| 133 | 19 | 7  | 17206 |
| 134 | 2  | 67 | 6     |
| 134 | 67 | 2  | 1     |
| 135 | 3  | 45 | 47    |
| 135 | 5  | 27 | 676   |
| 135 | 9  | 15 | 6807  |
| 135 | 15 | 9  | 18656 |
| 135 | 27 | 5  | 10717 |
| 135 | 45 | 3  | 711   |
| 136 | 2  | 68 | 5     |
| 136 | 4  | 34 | 239   |

|     |    |    |       |
|-----|----|----|-------|
| 136 | 8  | 17 | 4763  |
| 136 | 17 | 8  | 18430 |
| 136 | 34 | 4  | 4802  |
| 136 | 68 | 2  | 1     |
| 138 | 2  | 69 | 8     |
| 138 | 3  | 46 | 5     |
| 138 | 6  | 23 | 1599  |
| 138 | 23 | 6  | 17628 |
| 138 | 46 | 3  | 776   |
| 138 | 69 | 2  | 1     |
| 140 | 2  | 70 | 7     |
| 140 | 4  | 35 | 241   |
| 140 | 5  | 28 | 234   |
| 140 | 7  | 20 | 1599  |
| 140 | 10 | 14 | 11065 |
| 140 | 14 | 10 | 21981 |
| 140 | 20 | 7  | 24422 |
| 140 | 28 | 5  | 13391 |
| 140 | 35 | 4  | 5561  |
| 140 | 70 | 2  | 1     |
| 141 | 3  | 47 | 49    |
| 141 | 47 | 3  | 859   |
| 142 | 2  | 71 | 8     |
| 142 | 71 | 2  | 1     |
| 143 | 11 | 13 | 15893 |
| 143 | 13 | 11 | 22512 |
| 144 | 2  | 72 | 11    |
| 144 | 3  | 48 | 8     |
| 144 | 4  | 36 | 258   |
| 144 | 6  | 24 | 1840  |
| 144 | 8  | 18 | 6143  |
| 144 | 9  | 16 | 5730  |
| 144 | 12 | 12 | 20164 |
| 144 | 16 | 9  | 30055 |
| 144 | 18 | 8  | 31279 |
| 144 | 24 | 6  | 24581 |
| 144 | 36 | 4  | 6585  |
| 144 | 48 | 3  | 943   |
| 144 | 72 | 2  | 1     |
| 145 | 5  | 29 | 787   |
| 145 | 29 | 5  | 16663 |
| 146 | 2  | 73 | 6     |
| 146 | 73 | 2  | 1     |
| 147 | 3  | 49 | 55    |
| 147 | 7  | 21 | 3902  |
| 147 | 21 | 7  | 34451 |
| 147 | 49 | 3  | 1028  |

|     |    |    |       |
|-----|----|----|-------|
| 148 | 2  | 74 | 5     |
| 148 | 4  | 37 | 283   |
| 148 | 37 | 4  | 7623  |
| 148 | 74 | 2  | 1     |
| 150 | 2  | 75 | 12    |
| 150 | 3  | 50 | 5     |
| 150 | 5  | 30 | 283   |
| 150 | 6  | 25 | 2109  |
| 150 | 10 | 15 | 15767 |
| 150 | 15 | 10 | 31296 |
| 150 | 25 | 6  | 30965 |
| 150 | 30 | 5  | 20651 |
| 150 | 50 | 3  | 1135  |
| 150 | 75 | 2  | 1     |
| 152 | 2  | 76 | 4     |
| 152 | 4  | 38 | 281   |
| 152 | 8  | 19 | 7715  |
| 152 | 19 | 8  | 42173 |
| 152 | 38 | 4  | 8930  |
| 152 | 76 | 2  | 1     |
| 153 | 3  | 51 | 60    |
| 153 | 9  | 17 | 12294 |
| 153 | 17 | 9  | 47737 |
| 153 | 51 | 3  | 1243  |
| 154 | 2  | 77 | 8     |
| 154 | 7  | 22 | 2246  |
| 154 | 11 | 14 | 16875 |
| 154 | 14 | 11 | 40385 |
| 154 | 22 | 7  | 48169 |
| 154 | 77 | 2  | 1     |
| 155 | 5  | 31 | 961   |
| 155 | 31 | 5  | 25488 |
| 156 | 2  | 78 | 11    |
| 156 | 3  | 52 | 8     |
| 156 | 4  | 39 | 308   |
| 156 | 6  | 26 | 2402  |
| 156 | 12 | 13 | 32137 |
| 156 | 13 | 12 | 29782 |
| 156 | 26 | 6  | 42498 |
| 156 | 39 | 4  | 10318 |
| 156 | 52 | 3  | 1352  |
| 156 | 78 | 2  | 1     |
| 158 | 2  | 79 | 5     |
| 158 | 79 | 2  | 1     |
| 159 | 3  | 53 | 58    |
| 159 | 53 | 3  | 1485  |
| 160 | 2  | 80 | 8     |

|     |    |    |       |
|-----|----|----|-------|
| 160 | 4  | 40 | 335   |
| 160 | 5  | 32 | 303   |
| 160 | 8  | 20 | 9631  |
| 160 | 10 | 16 | 22098 |
| 160 | 16 | 10 | 62383 |
| 160 | 20 | 8  | 68774 |
| 160 | 32 | 5  | 31360 |
| 160 | 40 | 4  | 12068 |
| 160 | 80 | 2  | 1     |
| 161 | 7  | 23 | 5558  |
| 161 | 23 | 7  | 66625 |
| 162 | 2  | 81 | 10    |
| 162 | 3  | 54 | 8     |
| 162 | 6  | 27 | 2735  |
| 162 | 9  | 18 | 9631  |
| 162 | 18 | 9  | 74509 |
| 162 | 27 | 6  | 53186 |
| 162 | 54 | 3  | 1623  |
| 162 | 81 | 2  | 1     |
| 164 | 2  | 82 | 5     |
| 164 | 4  | 41 | 335   |
| 164 | 41 | 4  | 13843 |
| 164 | 82 | 2  | 1     |
| 165 | 3  | 55 | 60    |
| 165 | 5  | 33 | 1168  |
| 165 | 11 | 15 | 35174 |
| 165 | 15 | 11 | 70868 |
| 165 | 33 | 5  | 38432 |
| 165 | 55 | 3  | 1764  |
| 166 | 2  | 83 | 6     |
| 166 | 83 | 2  | 1     |
| 168 | 2  | 84 | 13    |
| 168 | 3  | 56 | 6     |
| 168 | 4  | 42 | 360   |
| 168 | 6  | 28 | 3087  |
| 168 | 7  | 24 | 2995  |
| 168 | 8  | 21 | 12037 |
| 168 | 12 | 14 | 49767 |
| 168 | 14 | 12 | 71086 |
| 168 | 21 | 8  | 91854 |
| 168 | 24 | 7  | 91622 |
| 168 | 28 | 6  | 71702 |
| 168 | 42 | 4  | 16123 |
| 168 | 56 | 3  | 1934  |
| 168 | 84 | 2  | 1     |
| 169 | 13 | 13 | 63114 |
| 170 | 2  | 85 | 9     |

|     |    |    |        |
|-----|----|----|--------|
| 170 | 5  | 34 | 360    |
| 170 | 10 | 17 | 30243  |
| 170 | 17 | 10 | 87706  |
| 170 | 34 | 5  | 46963  |
| 170 | 85 | 2  | 1      |
| 171 | 3  | 57 | 65     |
| 171 | 9  | 19 | 21040  |
| 171 | 19 | 9  | 114825 |
| 171 | 57 | 3  | 2107   |
| 172 | 2  | 86 | 6      |
| 172 | 4  | 43 | 382    |
| 172 | 43 | 4  | 18500  |
| 172 | 86 | 2  | 1      |
| 174 | 2  | 87 | 11     |
| 174 | 3  | 58 | 6      |
| 174 | 6  | 29 | 3484   |
| 174 | 29 | 6  | 89365  |
| 174 | 58 | 3  | 2283   |
| 174 | 87 | 2  | 1      |
| 175 | 5  | 35 | 1332   |
| 175 | 7  | 25 | 7784   |
| 175 | 25 | 7  | 125121 |
| 175 | 35 | 5  | 57187  |
| 176 | 2  | 88 | 7      |
| 176 | 4  | 44 | 385    |
| 176 | 8  | 22 | 14716  |
| 176 | 11 | 16 | 34220  |
| 176 | 16 | 11 | 121915 |
| 176 | 22 | 8  | 144873 |
| 176 | 44 | 4  | 21388  |
| 176 | 88 | 2  | 1      |
| 177 | 3  | 59 | 69     |
| 177 | 59 | 3  | 2497   |
| 178 | 2  | 89 | 7      |
| 178 | 89 | 2  | 1      |
| 180 | 2  | 90 | 14     |
| 180 | 3  | 60 | 7      |
| 180 | 4  | 45 | 421    |
| 180 | 5  | 36 | 411    |
| 180 | 6  | 30 | 3902   |
| 180 | 9  | 20 | 15426  |
| 180 | 10 | 18 | 40940  |
| 180 | 12 | 15 | 75208  |
| 180 | 15 | 12 | 103784 |
| 180 | 18 | 10 | 164580 |
| 180 | 20 | 9  | 175022 |
| 180 | 30 | 6  | 118725 |

|     |    |    |        |
|-----|----|----|--------|
| 180 | 36 | 5  | 69441  |
| 180 | 45 | 4  | 24473  |
| 180 | 60 | 3  | 2716   |
| 180 | 90 | 2  | 1      |
| 182 | 2  | 91 | 6      |
| 182 | 7  | 26 | 3902   |
| 182 | 13 | 14 | 75208  |
| 182 | 14 | 13 | 120273 |
| 182 | 26 | 7  | 169419 |
| 182 | 91 | 2  | 1      |
| 183 | 3  | 61 | 75     |
| 183 | 61 | 3  | 2941   |
| 184 | 2  | 92 | 8      |
| 184 | 4  | 46 | 445    |
| 184 | 8  | 23 | 17888  |
| 184 | 23 | 8  | 191870 |
| 184 | 46 | 4  | 28261  |
| 184 | 92 | 2  | 1      |
| 185 | 5  | 37 | 1577   |
| 185 | 37 | 5  | 84070  |
| 186 | 2  | 93 | 13     |
| 186 | 3  | 62 | 8      |
| 186 | 6  | 31 | 4367   |
| 186 | 31 | 6  | 146915 |
| 186 | 62 | 3  | 3207   |
| 186 | 93 | 2  | 1      |
| 187 | 11 | 17 | 71148  |
| 187 | 17 | 11 | 205945 |
| 188 | 2  | 94 | 5      |
| 188 | 4  | 47 | 437    |
| 188 | 47 | 4  | 32166  |
| 188 | 94 | 2  | 1      |
| 189 | 3  | 63 | 74     |
| 189 | 7  | 27 | 10511  |
| 189 | 9  | 21 | 34355  |
| 189 | 21 | 9  | 263175 |
| 189 | 27 | 7  | 228179 |
| 189 | 63 | 3  | 3477   |
| 190 | 2  | 95 | 8      |
| 190 | 5  | 38 | 437    |
| 190 | 10 | 19 | 54755  |
| 190 | 19 | 10 | 229625 |
| 190 | 38 | 5  | 101500 |
| 190 | 95 | 2  | 1      |
| 192 | 2  | 96 | 11     |
| 192 | 3  | 64 | 8      |
| 192 | 4  | 48 | 482    |

|     |     |     |        |
|-----|-----|-----|--------|
| 192 | 6   | 32  | 4861   |
| 192 | 8   | 24  | 21794  |
| 192 | 12  | 16  | 111162 |
| 192 | 16  | 12  | 227653 |
| 192 | 24  | 8   | 294168 |
| 192 | 32  | 6   | 193107 |
| 192 | 48  | 4   | 37019  |
| 192 | 64  | 3   | 3759   |
| 192 | 96  | 2   | 1      |
| 194 | 2   | 97  | 7      |
| 194 | 97  | 2   | 1      |
| 195 | 3   | 65  | 73     |
| 195 | 5   | 39  | 1861   |
| 195 | 13  | 15  | 156247 |
| 195 | 15  | 13  | 223955 |
| 195 | 39  | 5   | 122221 |
| 195 | 65  | 3   | 4092   |
| 196 | 2   | 98  | 9      |
| 196 | 4   | 49  | 508    |
| 196 | 7   | 28  | 5140   |
| 196 | 14  | 14  | 197319 |
| 196 | 28  | 7   | 305575 |
| 196 | 49  | 4   | 42116  |
| 196 | 98  | 2   | 1      |
| 198 | 2   | 99  | 13     |
| 198 | 3   | 66  | 9      |
| 198 | 6   | 33  | 5415   |
| 198 | 9   | 22  | 23746  |
| 198 | 11  | 18  | 64682  |
| 198 | 18  | 11  | 342132 |
| 198 | 22  | 9   | 391903 |
| 198 | 33  | 6   | 237612 |
| 198 | 66  | 3   | 4431   |
| 198 | 99  | 2   | 1      |
| 200 | 2   | 100 | 8      |
| 200 | 4   | 50  | 503    |
| 200 | 5   | 40  | 509    |
| 200 | 8   | 25  | 26104  |
| 200 | 10  | 20  | 71891  |
| 200 | 20  | 10  | 410506 |
| 200 | 25  | 8   | 386457 |
| 200 | 40  | 5   | 146794 |
| 200 | 50  | 4   | 48205  |
| 200 | 100 | 2   | 1      |
| 201 | 3   | 67  | 82     |
| 201 | 67  | 3   | 4783   |
| 202 | 2   | 101 | 9      |

|     |     |     |        |
|-----|-----|-----|--------|
| 202 | 101 | 2   | 1      |
| 203 | 7   | 29  | 13903  |
| 203 | 29  | 7   | 406413 |
| 204 | 2   | 102 | 14     |
| 204 | 3   | 68  | 9      |
| 204 | 4   | 51  | 556    |
| 204 | 6   | 34  | 5994   |
| 204 | 12  | 17  | 161139 |
| 204 | 17  | 12  | 329585 |
| 204 | 34  | 6   | 308554 |
| 204 | 51  | 4   | 54721  |
| 204 | 68  | 3   | 5191   |
| 204 | 102 | 2   | 1      |
| 205 | 5   | 41  | 2077   |
| 205 | 41  | 5   | 175865 |
| 206 | 2   | 103 | 7      |
| 206 | 103 | 2   | 1      |
| 207 | 3   | 69  | 85     |
| 207 | 9   | 23  | 54010  |
| 207 | 23  | 9   | 578025 |
| 207 | 69  | 3   | 5610   |
| 208 | 2   | 104 | 7      |
| 208 | 4   | 52  | 571    |
| 208 | 8   | 26  | 31083  |
| 208 | 13  | 16  | 171417 |
| 208 | 16  | 13  | 408522 |
| 208 | 26  | 8   | 578304 |
| 208 | 52  | 4   | 62546  |
| 208 | 104 | 2   | 1      |
| 209 | 11  | 19  | 135407 |
| 209 | 19  | 11  | 559689 |
| 210 | 2   | 105 | 19     |
| 210 | 3   | 70  | 7      |
| 210 | 5   | 42  | 571    |
| 210 | 6   | 35  | 6635   |
| 210 | 7   | 30  | 6493   |
| 210 | 10  | 21  | 93843  |
| 210 | 14  | 15  | 315413 |
| 210 | 15  | 14  | 295081 |
| 210 | 21  | 10  | 566612 |
| 210 | 30  | 7   | 537942 |
| 210 | 35  | 6   | 378174 |
| 210 | 42  | 5   | 210219 |
| 210 | 70  | 3   | 6050   |
| 210 | 105 | 2   | 1      |
| 212 | 2   | 106 | 6      |
| 212 | 4   | 53  | 561    |

|     |     |     |        |
|-----|-----|-----|--------|
| 212 | 53  | 4   | 70721  |
| 212 | 106 | 2   | 1      |
| 213 | 3   | 71  | 95     |
| 213 | 71  | 3   | 6557   |
| 214 | 2   | 107 | 8      |
| 214 | 107 | 2   | 1      |
| 215 | 5   | 43  | 2417   |
| 215 | 43  | 5   | 250675 |
| 216 | 2   | 108 | 13     |
| 216 | 3   | 72  | 8      |
| 216 | 4   | 54  | 632    |
| 216 | 6   | 36  | 7301   |
| 216 | 8   | 27  | 37101  |
| 216 | 9   | 24  | 35352  |
| 216 | 12  | 18  | 229545 |
| 216 | 18  | 12  | 675679 |
| 216 | 24  | 9   | 843771 |
| 216 | 27  | 8   | 754162 |
| 216 | 36  | 6   | 486084 |
| 216 | 54  | 4   | 80591  |
| 216 | 72  | 3   | 7074   |
| 216 | 108 | 2   | 1      |
| 217 | 7   | 31  | 18340  |
| 217 | 31  | 7   | 708621 |
| 218 | 2   | 109 | 7      |
| 218 | 109 | 2   | 1      |
| 219 | 3   | 73  | 88     |
| 219 | 73  | 3   | 7615   |
| 220 | 2   | 110 | 9      |
| 220 | 4   | 55  | 657    |
| 220 | 5   | 44  | 598    |
| 220 | 10  | 22  | 121073 |
| 220 | 11  | 20  | 114906 |
| 220 | 20  | 11  | 902671 |
| 220 | 22  | 10  | 974443 |
| 220 | 44  | 5   | 298299 |
| 220 | 55  | 4   | 91072  |
| 220 | 110 | 2   | 1      |
| 221 | 13  | 17  | 352520 |
| 221 | 17  | 13  | 729068 |
| 222 | 2   | 111 | 11     |
| 222 | 3   | 74  | 9      |
| 222 | 6   | 37  | 8041   |
| 222 | 37  | 6   | 592629 |
| 222 | 74  | 3   | 8236   |
| 222 | 111 | 2   | 1      |
| 224 | 2   | 112 | 7      |

|     |     |     |         |
|-----|-----|-----|---------|
| 224 | 4   | 56  | 645     |
| 224 | 7   | 32  | 8041    |
| 224 | 8   | 28  | 43734   |
| 224 | 14  | 16  | 490938  |
| 224 | 16  | 14  | 706922  |
| 224 | 28  | 8   | 1104949 |
| 224 | 32  | 7   | 928161  |
| 224 | 56  | 4   | 103367  |
| 224 | 112 | 2   | 1       |
| 225 | 3   | 75  | 90      |
| 225 | 5   | 45  | 2778    |
| 225 | 9   | 25  | 82181   |
| 225 | 15  | 15  | 619015  |
| 225 | 25  | 9   | 1221620 |
| 225 | 45  | 5   | 354179  |
| 225 | 75  | 3   | 8872    |
| 226 | 2   | 113 | 7       |
| 226 | 113 | 2   | 1       |
| 228 | 2   | 114 | 12      |
| 228 | 3   | 76  | 7       |
| 228 | 4   | 57  | 705     |
| 228 | 6   | 38  | 8820    |
| 228 | 12  | 19  | 321848  |
| 228 | 19  | 12  | 967764  |
| 228 | 38  | 6   | 755490  |
| 228 | 57  | 4   | 116534  |
| 228 | 76  | 3   | 9543    |
| 228 | 114 | 2   | 1       |
| 230 | 2   | 115 | 9       |
| 230 | 5   | 46  | 705     |
| 230 | 10  | 23  | 154248  |
| 230 | 23  | 10  | 1332468 |
| 230 | 46  | 5   | 419696  |
| 230 | 115 | 2   | 1       |
| 231 | 3   | 77  | 94      |
| 231 | 7   | 33  | 23612   |
| 231 | 11  | 21  | 243949  |
| 231 | 21  | 11  | 1436849 |
| 231 | 33  | 7   | 1210488 |
| 231 | 77  | 3   | 10303   |
| 232 | 2   | 116 | 7       |
| 232 | 4   | 58  | 726     |
| 232 | 8   | 29  | 51205   |
| 232 | 29  | 8   | 1430846 |
| 232 | 58  | 4   | 132113  |
| 232 | 116 | 2   | 1       |
| 234 | 2   | 117 | 15      |

|     |     |     |         |
|-----|-----|-----|---------|
| 234 | 3   | 78  | 7       |
| 234 | 6   | 39  | 9663    |
| 234 | 9   | 26  | 51205   |
| 234 | 13  | 18  | 359412  |
| 234 | 18  | 13  | 1277951 |
| 234 | 26  | 9   | 1754615 |
| 234 | 39  | 6   | 916739  |
| 234 | 78  | 3   | 11079   |
| 234 | 117 | 2   | 1       |
| 235 | 5   | 47  | 3076    |
| 235 | 47  | 5   | 496332  |
| 236 | 2   | 118 | 9       |
| 236 | 4   | 59  | 713     |
| 236 | 59  | 4   | 148496  |
| 236 | 118 | 2   | 1       |
| 237 | 3   | 79  | 102     |
| 237 | 79  | 3   | 11901   |
| 238 | 2   | 119 | 9       |
| 238 | 7   | 34  | 10095   |
| 238 | 14  | 17  | 747910  |
| 238 | 17  | 14  | 1046015 |
| 238 | 34  | 7   | 1572162 |
| 238 | 119 | 2   | 1       |
| 240 | 2   | 120 | 18      |
| 240 | 3   | 80  | 9       |
| 240 | 4   | 60  | 793     |
| 240 | 5   | 48  | 755     |
| 240 | 6   | 40  | 10556   |
| 240 | 8   | 30  | 60132   |
| 240 | 10  | 24  | 195566  |
| 240 | 12  | 20  | 444881  |
| 240 | 15  | 16  | 747910  |
| 240 | 16  | 15  | 1188224 |
| 240 | 20  | 12  | 1880759 |
| 240 | 24  | 10  | 2213942 |
| 240 | 30  | 8   | 2057975 |
| 240 | 40  | 6   | 1158735 |
| 240 | 48  | 5   | 585840  |
| 240 | 60  | 4   | 167893  |
| 240 | 80  | 3   | 12829   |
| 240 | 120 | 2   | 1       |
| 242 | 2   | 121 | 8       |
| 242 | 11  | 22  | 195566  |
| 242 | 22  | 11  | 2259337 |
| 242 | 121 | 2   | 1       |
| 243 | 3   | 81  | 109     |
| 243 | 9   | 27  | 121624  |

|     |     |     |         |
|-----|-----|-----|---------|
| 243 | 27  | 9   | 2499012 |
| 243 | 81  | 3   | 13781   |
| 244 | 2   | 122 | 9       |
| 244 | 4   | 61  | 815     |
| 244 | 61  | 4   | 188587  |
| 244 | 122 | 2   | 1       |
| 245 | 5   | 49  | 3523    |
| 245 | 7   | 35  | 29834   |
| 245 | 35  | 7   | 2032144 |
| 245 | 49  | 5   | 690210  |
| 246 | 2   | 123 | 16      |
| 246 | 3   | 82  | 9       |
| 246 | 6   | 41  | 11511   |
| 246 | 41  | 6   | 1401064 |
| 246 | 82  | 3   | 14786   |
| 246 | 123 | 2   | 1       |
| 247 | 13  | 19  | 739519  |
| 247 | 19  | 13  | 2203730 |
| 248 | 2   | 124 | 6       |
| 248 | 4   | 62  | 783     |
| 248 | 8   | 31  | 69968   |
| 248 | 31  | 8   | 2647827 |
| 248 | 62  | 4   | 212538  |
| 248 | 124 | 2   | 1       |
| 249 | 3   | 83  | 108     |
| 249 | 83  | 3   | 15910   |
| 250 | 2   | 125 | 9       |
| 250 | 5   | 50  | 783     |
| 250 | 10  | 25  | 245622  |
| 250 | 25  | 10  | 3003610 |
| 250 | 50  | 5   | 811710  |
| 250 | 125 | 2   | 1       |
| 252 | 2   | 126 | 16      |
| 252 | 3   | 84  | 9       |
| 252 | 4   | 63  | 877     |
| 252 | 6   | 42  | 12516   |
| 252 | 7   | 36  | 12361   |
| 252 | 9   | 28  | 72304   |
| 252 | 12  | 21  | 606938  |
| 252 | 14  | 18  | 1118677 |
| 252 | 18  | 14  | 2327972 |
| 252 | 21  | 12  | 2665109 |
| 252 | 28  | 9   | 3534991 |
| 252 | 36  | 7   | 2616602 |
| 252 | 42  | 6   | 1757193 |
| 252 | 63  | 4   | 238258  |
| 252 | 84  | 3   | 17066   |

|     |     |     |         |
|-----|-----|-----|---------|
| 252 | 126 | 2   | 1       |
| 253 | 11  | 23  | 419301  |
| 253 | 23  | 11  | 3512327 |
| 254 | 2   | 127 | 9       |
| 254 | 127 | 2   | 1       |
| 255 | 3   | 85  | 108     |
| 255 | 5   | 51  | 3958    |
| 255 | 15  | 17  | 1542921 |
| 255 | 17  | 15  | 2231187 |
| 255 | 51  | 5   | 952921  |
| 255 | 85  | 3   | 18292   |
| 256 | 2   | 128 | 8       |
| 256 | 4   | 64  | 899     |
| 256 | 8   | 32  | 80777   |
| 256 | 16  | 16  | 1944066 |
| 256 | 32  | 8   | 3746422 |
| 256 | 64  | 4   | 268215  |
| 256 | 128 | 2   | 1       |
| 258 | 2   | 129 | 14      |
| 258 | 3   | 86  | 8       |
| 258 | 6   | 43  | 13611   |
| 258 | 43  | 6   | 2115863 |
| 258 | 86  | 3   | 19659   |
| 258 | 129 | 2   | 1       |
| 259 | 7   | 37  | 37678   |
| 259 | 37  | 7   | 3356909 |
| 260 | 2   | 130 | 10      |
| 260 | 4   | 65  | 886     |
| 260 | 5   | 52  | 923     |
| 260 | 10  | 26  | 305409  |
| 260 | 13  | 20  | 705640  |
| 260 | 20  | 13  | 3738867 |
| 260 | 26  | 10  | 4846564 |
| 260 | 52  | 5   | 1116847 |
| 260 | 65  | 4   | 299924  |
| 260 | 130 | 2   | 1       |
| 261 | 3   | 87  | 111     |
| 261 | 9   | 29  | 175658  |
| 261 | 29  | 9   | 4965932 |
| 261 | 87  | 3   | 21062   |
| 262 | 2   | 131 | 9       |
| 262 | 131 | 2   | 1       |
| 264 | 2   | 132 | 16      |
| 264 | 3   | 88  | 9       |
| 264 | 4   | 66  | 979     |
| 264 | 6   | 44  | 14761   |
| 264 | 8   | 33  | 93592   |

|     |     |     |         |
|-----|-----|-----|---------|
| 264 | 11  | 24  | 319488  |
| 264 | 12  | 22  | 818186  |
| 264 | 22  | 12  | 4948021 |
| 264 | 24  | 11  | 5402221 |
| 264 | 33  | 8   | 4790718 |
| 264 | 44  | 6   | 2636781 |
| 264 | 66  | 4   | 336864  |
| 264 | 88  | 3   | 22547   |
| 264 | 132 | 2   | 1       |
| 265 | 5   | 53  | 4328    |
| 265 | 53  | 5   | 1306772 |
| 266 | 2   | 133 | 8       |
| 266 | 7   | 38  | 14761   |
| 266 | 14  | 19  | 1642587 |
| 266 | 19  | 14  | 3408989 |
| 266 | 38  | 7   | 4289057 |
| 266 | 133 | 2   | 1       |
| 267 | 3   | 89  | 120     |
| 267 | 89  | 3   | 24196   |
| 268 | 2   | 134 | 9       |
| 268 | 4   | 67  | 981     |
| 268 | 67  | 4   | 376398  |
| 268 | 134 | 2   | 1       |
| 270 | 2   | 135 | 19      |
| 270 | 3   | 90  | 9       |
| 270 | 5   | 54  | 981     |
| 270 | 6   | 45  | 15987   |
| 270 | 9   | 30  | 100071  |
| 270 | 10  | 27  | 378571  |
| 270 | 15  | 18  | 1731924 |
| 270 | 18  | 15  | 4104452 |
| 270 | 27  | 10  | 6520323 |
| 270 | 30  | 9   | 6928378 |
| 270 | 45  | 6   | 3162474 |
| 270 | 54  | 5   | 1526624 |
| 270 | 90  | 3   | 25895   |
| 270 | 135 | 2   | 1       |
| 272 | 2   | 136 | 7       |
| 272 | 4   | 68  | 958     |
| 272 | 8   | 34  | 107672  |
| 272 | 16  | 17  | 3103663 |
| 272 | 17  | 16  | 2931683 |
| 272 | 34  | 8   | 6680069 |
| 272 | 68  | 4   | 421695  |
| 272 | 136 | 2   | 1       |
| 273 | 3   | 91  | 127     |
| 273 | 7   | 39  | 46914   |

|     |     |     |          |
|-----|-----|-----|----------|
| 273 | 13  | 21  | 1457604  |
| 273 | 21  | 13  | 6251754  |
| 273 | 39  | 7   | 5461103  |
| 273 | 91  | 3   | 27697    |
| 274 | 2   | 137 | 11       |
| 274 | 137 | 2   | 1        |
| 275 | 5   | 55  | 4930     |
| 275 | 11  | 25  | 695610   |
| 275 | 25  | 11  | 8226292  |
| 275 | 55  | 5   | 1780641  |
| 276 | 2   | 138 | 16       |
| 276 | 3   | 92  | 11       |
| 276 | 4   | 69  | 1084     |
| 276 | 6   | 46  | 17263    |
| 276 | 12  | 23  | 1090924  |
| 276 | 23  | 12  | 6949849  |
| 276 | 46  | 6   | 3915558  |
| 276 | 69  | 4   | 470308   |
| 276 | 92  | 3   | 29683    |
| 276 | 138 | 2   | 1        |
| 278 | 2   | 139 | 7        |
| 278 | 139 | 2   | 1        |
| 279 | 3   | 93  | 122      |
| 279 | 9   | 31  | 248401   |
| 279 | 31  | 9   | 9608991  |
| 279 | 93  | 3   | 31726    |
| 280 | 2   | 140 | 14       |
| 280 | 4   | 70  | 1093     |
| 280 | 5   | 56  | 1001     |
| 280 | 7   | 40  | 17931    |
| 280 | 8   | 35  | 122897   |
| 280 | 10  | 28  | 465078   |
| 280 | 14  | 20  | 2372614  |
| 280 | 20  | 14  | 7141800  |
| 280 | 28  | 10  | 10261578 |
| 280 | 35  | 8   | 8493626  |
| 280 | 40  | 7   | 6930997  |
| 280 | 56  | 5   | 2073856  |
| 280 | 70  | 4   | 526318   |
| 280 | 140 | 2   | 1        |
| 282 | 2   | 141 | 16       |
| 282 | 3   | 94  | 14       |
| 282 | 6   | 47  | 18636    |
| 282 | 47  | 6   | 4681354  |
| 282 | 94  | 3   | 33897    |
| 282 | 141 | 2   | 1        |
| 284 | 2   | 142 | 8        |

|     |     |     |          |
|-----|-----|-----|----------|
| 284 | 4   | 71  | 1071     |
| 284 | 71  | 4   | 585855   |
| 284 | 142 | 2   | 1        |
| 285 | 3   | 95  | 129      |
| 285 | 5   | 57  | 5425     |
| 285 | 15  | 19  | 3542433  |
| 285 | 19  | 15  | 7418237  |
| 285 | 57  | 5   | 2411791  |
| 285 | 95  | 3   | 36287    |
| 286 | 2   | 143 | 12       |
| 286 | 11  | 26  | 503492   |
| 286 | 13  | 22  | 1315097  |
| 286 | 22  | 13  | 10317480 |
| 286 | 26  | 11  | 12409516 |
| 286 | 143 | 2   | 1        |
| 287 | 7   | 41  | 57295    |
| 287 | 41  | 7   | 8765283  |
| 288 | 2   | 144 | 17       |
| 288 | 3   | 96  | 12       |
| 288 | 4   | 72  | 1189     |
| 288 | 6   | 48  | 20081    |
| 288 | 8   | 36  | 140764   |
| 288 | 9   | 32  | 135790   |
| 288 | 12  | 24  | 1439801  |
| 288 | 16  | 18  | 4854284  |
| 288 | 18  | 16  | 7030222  |
| 288 | 24  | 12  | 12406615 |
| 288 | 32  | 9   | 13248239 |
| 288 | 36  | 8   | 11688914 |
| 288 | 48  | 6   | 5761288  |
| 288 | 72  | 4   | 654282   |
| 288 | 96  | 3   | 38750    |
| 288 | 144 | 2   | 1        |
| 289 | 17  | 17  | 6099684  |
| 290 | 2   | 145 | 10       |
| 290 | 5   | 58  | 1189     |
| 290 | 10  | 29  | 567348   |
| 290 | 29  | 10  | 13702750 |
| 290 | 58  | 5   | 2800812  |
| 290 | 145 | 2   | 1        |
| 291 | 3   | 97  | 134      |
| 291 | 97  | 3   | 41362    |
| 292 | 2   | 146 | 8        |
| 292 | 4   | 73  | 1184     |
| 292 | 73  | 4   | 727703   |
| 292 | 146 | 2   | 1        |
| 294 | 2   | 147 | 19       |



|     |     |     |          |
|-----|-----|-----|----------|
| 294 | 3   | 98  | 8        |
| 294 | 6   | 49  | 21640    |
| 294 | 7   | 42  | 21373    |
| 294 | 14  | 21  | 3381019  |
| 294 | 21  | 14  | 10353735 |
| 294 | 42  | 7   | 11050511 |
| 294 | 49  | 6   | 6864506  |
| 294 | 98  | 3   | 44220    |
| 294 | 147 | 2   | 1        |
| 295 | 5   | 59  | 5922     |
| 295 | 59  | 5   | 3248084  |
| 296 | 2   | 148 | 8        |
| 296 | 4   | 74  | 1167     |
| 296 | 8   | 37  | 160364   |
| 296 | 37  | 8   | 14782371 |
| 296 | 74  | 4   | 811029   |
| 296 | 148 | 2   | 1        |
| 297 | 3   | 99  | 143      |
| 297 | 9   | 33  | 344546   |
| 297 | 11  | 27  | 1115246  |
| 297 | 27  | 11  | 18554928 |
| 297 | 33  | 9   | 18159441 |
| 297 | 99  | 3   | 47172    |
| 298 | 2   | 149 | 11       |
| 298 | 149 | 2   | 1        |
| 299 | 13  | 23  | 2729537  |
| 299 | 23  | 13  | 16808424 |
| 300 | 2   | 150 | 21       |
| 300 | 3   | 100 | 11       |
| 300 | 4   | 75  | 1314     |
| 300 | 5   | 60  | 1232     |
| 300 | 6   | 50  | 23245    |
| 300 | 10  | 30  | 690016   |
| 300 | 12  | 25  | 1882456  |
| 300 | 15  | 20  | 3729418  |
| 300 | 20  | 15  | 13178681 |
| 300 | 25  | 12  | 17272172 |
| 300 | 30  | 10  | 21084354 |
| 300 | 50  | 6   | 8404322  |
| 300 | 60  | 5   | 3761699  |
| 300 | 75  | 4   | 900540   |
| 300 | 100 | 3   | 50309    |
| 300 | 150 | 2   | 1        |
| 301 | 7   | 43  | 70218    |
| 301 | 43  | 7   | 13891230 |
| 302 | 2   | 151 | 9        |
| 302 | 151 | 2   | 1        |

|     |     |     |          |
|-----|-----|-----|----------|
| 303 | 3   | 101 | 146      |
| 303 | 101 | 3   | 53732    |
| 304 | 2   | 152 | 10       |
| 304 | 4   | 76  | 1305     |
| 304 | 8   | 38  | 181357   |
| 304 | 16  | 19  | 7444425  |
| 304 | 19  | 16  | 10497192 |
| 304 | 38  | 8   | 20103624 |
| 304 | 76  | 4   | 1002626  |
| 304 | 152 | 2   | 1        |
| 305 | 5   | 61  | 6666     |
| 305 | 61  | 5   | 4350790  |
| 306 | 2   | 153 | 15       |
| 306 | 3   | 102 | 10       |
| 306 | 6   | 51  | 24966    |
| 306 | 9   | 34  | 181357   |
| 306 | 17  | 18  | 7444425  |
| 306 | 18  | 17  | 11736056 |
| 306 | 34  | 9   | 24763226 |
| 306 | 51  | 6   | 9980367  |
| 306 | 102 | 3   | 57263    |
| 306 | 153 | 2   | 1        |
| 308 | 2   | 154 | 8        |
| 308 | 4   | 77  | 1258     |
| 308 | 7   | 44  | 24966    |
| 308 | 11  | 28  | 773334   |
| 308 | 14  | 22  | 4751322  |
| 308 | 22  | 14  | 20616420 |
| 308 | 28  | 11  | 27512700 |
| 308 | 44  | 7   | 17407671 |
| 308 | 77  | 4   | 1111412  |
| 308 | 154 | 2   | 1        |
| 309 | 3   | 103 | 143      |
| 309 | 103 | 3   | 61010    |
| 310 | 2   | 155 | 12       |
| 310 | 5   | 62  | 1258     |
| 310 | 10  | 31  | 832920   |
| 310 | 31  | 10  | 27963022 |
| 310 | 62  | 5   | 5025743  |
| 310 | 155 | 2   | 1        |
| 312 | 2   | 156 | 17       |
| 312 | 3   | 104 | 12       |
| 312 | 4   | 78  | 1421     |
| 312 | 6   | 52  | 26725    |
| 312 | 8   | 39  | 205656   |
| 312 | 12  | 26  | 2439706  |
| 312 | 13  | 24  | 2339607  |

|     |     |     |          |
|-----|-----|-----|----------|
| 312 | 24  | 13  | 27061037 |
| 312 | 26  | 12  | 29826777 |
| 312 | 39  | 8   | 25295920 |
| 312 | 52  | 6   | 12157050 |
| 312 | 78  | 4   | 1235199  |
| 312 | 104 | 3   | 65088    |
| 312 | 156 | 2   | 1        |
| 314 | 2   | 157 | 9        |
| 314 | 157 | 2   | 1        |
| 315 | 3   | 105 | 146      |
| 315 | 5   | 63  | 7251     |
| 315 | 7   | 45  | 85172    |
| 315 | 9   | 35  | 470159   |
| 315 | 15  | 21  | 7602734  |
| 315 | 21  | 15  | 23042113 |
| 315 | 35  | 9   | 33594652 |
| 315 | 45  | 7   | 21752893 |
| 315 | 63  | 5   | 5798068  |
| 315 | 105 | 3   | 69306    |
| 316 | 2   | 158 | 10       |
| 316 | 4   | 79  | 1420     |
| 316 | 79  | 4   | 1368129  |
| 316 | 158 | 2   | 1        |
| 318 | 2   | 159 | 15       |
| 318 | 3   | 106 | 10       |
| 318 | 6   | 53  | 28645    |
| 318 | 53  | 6   | 14396222 |
| 318 | 106 | 3   | 73785    |
| 318 | 159 | 2   | 1        |
| 319 | 11  | 29  | 1736419  |
| 319 | 29  | 11  | 40473680 |
| 320 | 2   | 160 | 11       |
| 320 | 4   | 80  | 1393     |
| 320 | 5   | 64  | 1481     |
| 320 | 8   | 40  | 232348   |
| 320 | 10  | 32  | 999736   |
| 320 | 16  | 20  | 11215400 |
| 320 | 20  | 16  | 23574125 |
| 320 | 32  | 10  | 42188354 |
| 320 | 40  | 8   | 34033142 |
| 320 | 64  | 5   | 6681034  |
| 320 | 80  | 4   | 1517870  |
| 320 | 160 | 2   | 1        |
| 321 | 3   | 107 | 151      |
| 321 | 107 | 3   | 78638    |
| 322 | 2   | 161 | 11       |
| 322 | 7   | 46  | 29545    |

|     |     |     |          |
|-----|-----|-----|----------|
| 322 | 14  | 23  | 6592873  |
| 322 | 23  | 14  | 29604013 |
| 322 | 46  | 7   | 27111712 |
| 322 | 161 | 2   | 1        |
| 323 | 17  | 19  | 15260991 |
| 323 | 19  | 17  | 22141519 |
| 324 | 2   | 162 | 20       |
| 324 | 3   | 108 | 11       |
| 324 | 4   | 81  | 1562     |
| 324 | 6   | 54  | 30640    |
| 324 | 9   | 36  | 238545   |
| 324 | 12  | 27  | 3136169  |
| 324 | 18  | 18  | 19144236 |
| 324 | 27  | 12  | 41171103 |
| 324 | 36  | 9   | 45348405 |
| 324 | 54  | 6   | 17450825 |
| 324 | 81  | 4   | 1678721  |
| 324 | 108 | 3   | 83655    |
| 324 | 162 | 2   | 1        |
| 325 | 5   | 65  | 7852     |
| 325 | 13  | 25  | 4899568  |
| 325 | 25  | 13  | 43096058 |
| 325 | 65  | 5   | 7689199  |
| 326 | 2   | 163 | 7        |
| 326 | 163 | 2   | 1        |
| 327 | 3   | 109 | 161      |
| 327 | 109 | 3   | 88982    |
| 328 | 2   | 164 | 10       |
| 328 | 4   | 82  | 1528     |
| 328 | 8   | 41  | 260657   |
| 328 | 41  | 8   | 42618735 |
| 328 | 82  | 4   | 1860598  |
| 328 | 164 | 2   | 1        |
| 329 | 7   | 47  | 101609   |
| 329 | 47  | 7   | 33696895 |
| 330 | 2   | 165 | 24       |
| 330 | 3   | 110 | 10       |
| 330 | 5   | 66  | 1528     |
| 330 | 6   | 55  | 32749    |
| 330 | 10  | 33  | 1197227  |
| 330 | 11  | 30  | 1154795  |
| 330 | 15  | 22  | 7560887  |
| 330 | 22  | 15  | 39713020 |
| 330 | 30  | 11  | 59096139 |
| 330 | 33  | 10  | 55575123 |
| 330 | 55  | 6   | 20605208 |
| 330 | 66  | 5   | 8839319  |

|     |     |     |          |
|-----|-----|-----|----------|
| 330 | 110 | 3   | 94747    |
| 330 | 165 | 2   | 1        |
| 332 | 2   | 166 | 6        |
| 332 | 4   | 83  | 1477     |
| 332 | 83  | 4   | 2054877  |
| 332 | 166 | 2   | 1        |
| 333 | 3   | 111 | 167      |
| 333 | 9   | 37  | 631628   |
| 333 | 37  | 9   | 60935895 |
| 333 | 111 | 3   | 100713   |
| 334 | 2   | 167 | 11       |
| 334 | 167 | 2   | 1        |
| 335 | 5   | 67  | 8782     |
| 335 | 67  | 5   | 10149889 |
| 336 | 2   | 168 | 19       |
| 336 | 3   | 112 | 11       |
| 336 | 4   | 84  | 1688     |
| 336 | 6   | 56  | 34932    |
| 336 | 7   | 48  | 34627    |
| 336 | 8   | 42  | 293000   |
| 336 | 12  | 28  | 4000809  |
| 336 | 14  | 24  | 9050491  |
| 336 | 16  | 21  | 16637213 |
| 336 | 21  | 16  | 34833767 |
| 336 | 24  | 14  | 56454712 |
| 336 | 28  | 12  | 69060617 |
| 336 | 42  | 8   | 56778134 |
| 336 | 48  | 7   | 41774608 |
| 336 | 56  | 6   | 24870913 |
| 336 | 84  | 4   | 2273926  |
| 336 | 112 | 3   | 107042   |
| 336 | 168 | 2   | 1        |
| 338 | 2   | 169 | 9        |
| 338 | 13  | 26  | 4000809  |
| 338 | 26  | 13  | 67914251 |
| 338 | 169 | 2   | 1        |
| 339 | 3   | 113 | 161      |
| 339 | 113 | 3   | 113865   |
| 340 | 2   | 170 | 13       |
| 340 | 4   | 85  | 1664     |
| 340 | 5   | 68  | 1539     |
| 340 | 10  | 34  | 1423731  |
| 340 | 17  | 20  | 17454189 |
| 340 | 20  | 17  | 41022612 |
| 340 | 34  | 10  | 82391817 |
| 340 | 68  | 5   | 11641887 |
| 340 | 85  | 4   | 2509305  |

|     |     |     |          |
|-----|-----|-----|----------|
| 340 | 170 | 2   | 1        |
| 341 | 11  | 31  | 2641246  |
| 341 | 31  | 11  | 85675952 |
| 342 | 2   | 171 | 17       |
| 342 | 3   | 114 | 13       |
| 342 | 6   | 57  | 37231    |
| 342 | 9   | 38  | 309730   |
| 342 | 18  | 19  | 30585097 |
| 342 | 19  | 18  | 29066485 |
| 342 | 38  | 9   | 81512673 |
| 342 | 57  | 6   | 29282924 |
| 342 | 114 | 3   | 120933   |
| 342 | 171 | 2   | 1        |
| 343 | 7   | 49  | 121478   |
| 343 | 49  | 7   | 51665587 |
| 344 | 2   | 172 | 10       |
| 344 | 4   | 86  | 1626     |
| 344 | 8   | 43  | 328705   |
| 344 | 43  | 8   | 70781680 |
| 344 | 86  | 4   | 2772742  |
| 344 | 172 | 2   | 1        |
| 345 | 3   | 115 | 162      |
| 345 | 5   | 69  | 9431     |
| 345 | 15  | 23  | 15423687 |
| 345 | 23  | 15  | 67505080 |
| 345 | 69  | 5   | 13338742 |
| 345 | 115 | 3   | 128436   |
| 346 | 2   | 173 | 9        |
| 346 | 173 | 2   | 1        |
| 348 | 2   | 174 | 16       |
| 348 | 3   | 116 | 9        |
| 348 | 4   | 87  | 1814     |
| 348 | 6   | 58  | 39646    |
| 348 | 12  | 29  | 5067382  |
| 348 | 29  | 12  | 94592484 |
| 348 | 58  | 6   | 35198256 |
| 348 | 87  | 4   | 3055660  |
| 348 | 116 | 3   | 136512   |
| 348 | 174 | 2   | 1        |
| 350 | 2   | 175 | 13       |
| 350 | 5   | 70  | 1814     |
| 350 | 7   | 50  | 39646    |
| 350 | 10  | 35  | 1686207  |
| 350 | 14  | 25  | 12292295 |
| 350 | 25  | 14  | 80335204 |
| 350 | 35  | 10  | 1.08E+08 |
| 350 | 50  | 7   | 63739463 |

|     |     |     |          |
|-----|-----|-----|----------|
| 350 | 70  | 5   | 15266746 |
| 350 | 175 | 2   | 1        |
| 351 | 3   | 117 | 170      |
| 351 | 9   | 39  | 837365   |
| 351 | 13  | 27  | 8471308  |
| 351 | 27  | 13  | 1.06E+08 |
| 351 | 39  | 9   | 1.09E+08 |
| 351 | 117 | 3   | 144875   |
| 352 | 2   | 176 | 10       |
| 352 | 4   | 88  | 1781     |
| 352 | 8   | 44  | 366129   |
| 352 | 11  | 32  | 1686207  |
| 352 | 16  | 22  | 24311659 |
| 352 | 22  | 16  | 74027922 |
| 352 | 32  | 11  | 1.23E+08 |
| 352 | 44  | 8   | 93450980 |
| 352 | 88  | 4   | 3373293  |
| 352 | 176 | 2   | 1        |
| 354 | 2   | 177 | 20       |
| 354 | 3   | 118 | 10       |
| 354 | 6   | 59  | 42193    |
| 354 | 59  | 6   | 41338590 |
| 354 | 118 | 3   | 153740   |
| 354 | 177 | 2   | 1        |
| 355 | 5   | 71  | 10190    |
| 355 | 71  | 5   | 17455314 |
| 356 | 2   | 178 | 9        |
| 356 | 4   | 89  | 1745     |
| 356 | 89  | 4   | 3712917  |
| 356 | 178 | 2   | 1        |
| 357 | 3   | 119 | 180      |
| 357 | 7   | 51  | 144543   |
| 357 | 17  | 21  | 35471737 |
| 357 | 21  | 17  | 74733621 |
| 357 | 51  | 7   | 78451913 |
| 357 | 119 | 3   | 163263   |
| 358 | 2   | 179 | 10       |
| 358 | 179 | 2   | 1        |
| 360 | 2   | 180 | 22       |
| 360 | 3   | 120 | 10       |
| 360 | 4   | 90  | 1982     |
| 360 | 5   | 72  | 1843     |
| 360 | 6   | 60  | 44846    |
| 360 | 8   | 45  | 408477   |
| 360 | 9   | 40  | 397250   |
| 360 | 10  | 36  | 1992416  |
| 360 | 12  | 30  | 6375319  |

|     |     |     |          |
|-----|-----|-----|----------|
| 360 | 15  | 24  | 14571054 |
| 360 | 18  | 20  | 47945132 |
| 360 | 20  | 18  | 69662487 |
| 360 | 24  | 15  | 1.13E+08 |
| 360 | 30  | 12  | 1.55E+08 |
| 360 | 36  | 10  | 1.57E+08 |
| 360 | 40  | 9   | 1.44E+08 |
| 360 | 45  | 8   | 1.16E+08 |
| 360 | 60  | 6   | 49491109 |
| 360 | 72  | 5   | 19937494 |
| 360 | 90  | 4   | 4093104  |
| 360 | 120 | 3   | 173137   |
| 360 | 180 | 2   | 1        |
| 361 | 19  | 19  | 60058289 |
| 362 | 2   | 181 | 8        |
| 362 | 181 | 2   | 1        |
| 363 | 3   | 121 | 182      |
| 363 | 11  | 33  | 3922860  |
| 363 | 33  | 11  | 1.77E+08 |
| 363 | 121 | 3   | 183608   |
| 364 | 2   | 182 | 14       |
| 364 | 4   | 91  | 1935     |
| 364 | 7   | 52  | 46006    |
| 364 | 13  | 28  | 6621541  |
| 364 | 14  | 26  | 16523969 |
| 364 | 26  | 14  | 1.48E+08 |
| 364 | 28  | 13  | 1.64E+08 |
| 364 | 52  | 7   | 96350402 |
| 364 | 91  | 4   | 4501713  |
| 364 | 182 | 2   | 1        |
| 365 | 5   | 73  | 11311    |
| 365 | 73  | 5   | 22749946 |
| 366 | 2   | 183 | 18       |
| 366 | 3   | 122 | 14       |
| 366 | 6   | 61  | 47616    |
| 366 | 61  | 6   | 57979499 |
| 366 | 122 | 3   | 194825   |
| 366 | 183 | 2   | 1        |
| 368 | 2   | 184 | 8        |
| 368 | 4   | 92  | 1849     |
| 368 | 8   | 46  | 455360   |
| 368 | 16  | 23  | 35047967 |
| 368 | 23  | 16  | 1.08E+08 |
| 368 | 46  | 8   | 1.52E+08 |
| 368 | 92  | 4   | 4956339  |
| 368 | 184 | 2   | 1        |
| 369 | 3   | 123 | 183      |

|     |     |     |          |
|-----|-----|-----|----------|
| 369 | 9   | 41  | 1096146  |
| 369 | 41  | 9   | 1.9E+08  |
| 369 | 123 | 3   | 206451   |
| 370 | 2   | 185 | 14       |
| 370 | 5   | 74  | 1849     |
| 370 | 10  | 37  | 2340194  |
| 370 | 37  | 10  | 2.05E+08 |
| 370 | 74  | 5   | 25934114 |
| 370 | 185 | 2   | 1        |
| 371 | 7   | 53  | 169135   |
| 371 | 53  | 7   | 1.18E+08 |
| 372 | 2   | 186 | 18       |
| 372 | 3   | 124 | 14       |
| 372 | 4   | 93  | 2104     |
| 372 | 6   | 62  | 50472    |
| 372 | 12  | 31  | 7970234  |
| 372 | 31  | 12  | 2.1E+08  |
| 372 | 62  | 6   | 69164560 |
| 372 | 93  | 4   | 5444518  |
| 372 | 124 | 3   | 218776   |
| 372 | 186 | 2   | 1        |
| 374 | 2   | 187 | 10       |
| 374 | 11  | 34  | 2417932  |
| 374 | 17  | 22  | 38336477 |
| 374 | 22  | 17  | 1.34E+08 |
| 374 | 34  | 11  | 2.51E+08 |
| 374 | 187 | 2   | 1        |
| 375 | 3   | 125 | 181      |
| 375 | 5   | 75  | 12015    |
| 375 | 15  | 25  | 29824605 |
| 375 | 25  | 15  | 1.88E+08 |
| 375 | 75  | 5   | 29535694 |
| 375 | 125 | 3   | 231966   |
| 376 | 2   | 188 | 11       |
| 376 | 4   | 94  | 2063     |
| 376 | 8   | 47  | 504024   |
| 376 | 47  | 8   | 1.88E+08 |
| 376 | 94  | 4   | 5989071  |
| 376 | 188 | 2   | 1        |
| 377 | 13  | 29  | 14169324 |
| 377 | 29  | 13  | 2.51E+08 |
| 378 | 2   | 189 | 22       |
| 378 | 3   | 126 | 11       |
| 378 | 6   | 63  | 53526    |
| 378 | 7   | 54  | 53065    |
| 378 | 9   | 42  | 504024   |
| 378 | 14  | 27  | 22021058 |

|     |     |     |          |
|-----|-----|-----|----------|
| 378 | 18  | 21  | 73871145 |
| 378 | 21  | 18  | 1.05E+08 |
| 378 | 27  | 14  | 2.08E+08 |
| 378 | 42  | 9   | 2.5E+08  |
| 378 | 54  | 7   | 1.44E+08 |
| 378 | 63  | 6   | 80826851 |
| 378 | 126 | 3   | 245648   |
| 378 | 189 | 2   | 1        |
| 380 | 2   | 190 | 13       |
| 380 | 4   | 95  | 2017     |
| 380 | 5   | 76  | 2181     |
| 380 | 10  | 38  | 2739460  |
| 380 | 19  | 20  | 73871145 |
| 380 | 20  | 19  | 1.16E+08 |
| 380 | 38  | 10  | 2.95E+08 |
| 380 | 76  | 5   | 33606306 |
| 380 | 95  | 4   | 6571847  |
| 380 | 190 | 2   | 1        |
| 381 | 3   | 127 | 195      |
| 381 | 127 | 3   | 260139   |
| 382 | 2   | 191 | 10       |
| 382 | 191 | 2   | 1        |
| 384 | 2   | 192 | 19       |
| 384 | 3   | 128 | 10       |
| 384 | 4   | 96  | 2283     |
| 384 | 6   | 64  | 56687    |
| 384 | 8   | 48  | 558657   |
| 384 | 12  | 32  | 9904795  |
| 384 | 16  | 24  | 49914239 |
| 384 | 24  | 16  | 2.2E+08  |
| 384 | 32  | 12  | 3.36E+08 |
| 384 | 48  | 8   | 2.44E+08 |
| 384 | 64  | 6   | 96085697 |
| 384 | 96  | 4   | 7220135  |
| 384 | 128 | 3   | 275605   |
| 384 | 192 | 2   | 1        |
| 385 | 5   | 77  | 12923    |
| 385 | 7   | 55  | 198449   |
| 385 | 11  | 35  | 5713310  |
| 385 | 35  | 11  | 3.55E+08 |
| 385 | 55  | 7   | 1.76E+08 |
| 385 | 77  | 5   | 38202960 |
| 386 | 2   | 193 | 12       |
| 386 | 193 | 2   | 1        |
| 387 | 3   | 129 | 200      |
| 387 | 9   | 43  | 1418891  |
| 387 | 43  | 9   | 3.28E+08 |

|     |     |     |          |
|-----|-----|-----|----------|
| 387 | 129 | 3   | 291658   |
| 388 | 2   | 194 | 9        |
| 388 | 4   | 97  | 2201     |
| 388 | 97  | 4   | 7916640  |
| 388 | 194 | 2   | 1        |
| 390 | 2   | 195 | 27       |
| 390 | 3   | 130 | 9        |
| 390 | 5   | 78  | 2201     |
| 390 | 6   | 65  | 60006    |
| 390 | 10  | 39  | 3200534  |
| 390 | 13  | 30  | 10640752 |
| 390 | 15  | 26  | 26886280 |
| 390 | 26  | 15  | 3.08E+08 |
| 390 | 30  | 13  | 3.82E+08 |
| 390 | 39  | 10  | 3.81E+08 |
| 390 | 65  | 6   | 1.12E+08 |
| 390 | 78  | 5   | 43389607 |
| 390 | 130 | 3   | 308664   |
| 390 | 195 | 2   | 1        |
| 391 | 17  | 23  | 77544998 |
| 391 | 23  | 17  | 2.37E+08 |
| 392 | 2   | 196 | 11       |
| 392 | 4   | 98  | 2116     |
| 392 | 7   | 56  | 60006    |
| 392 | 8   | 49  | 619151   |
| 392 | 14  | 28  | 29096131 |
