# Supplementary material for: Divisor Goldbach Conjecture and its Partition Number
Source: arXiv:1603.05233 source file (2016-03-14)
Supplement: Supplementary file 2 [file appendixII.pdf]

## Appendix II

| $n$ | $m$ | Divisor Goldbach partition |
|-----|-----|----------------------------|
| 4   | 2   | 2+2                        |
| 6   | 2   | 3+3                        |
| 6   | 3   | 2+2+2                      |
| 8   | 2   | 3+5                        |
| 8   | 4   | 2+2+2+2                    |
| 9   | 3   | 2+2+5                      |
| 9   | 3   | 3+3+3                      |
| 10  | 2   | 3+7                        |
| 10  | 2   | 5+5                        |
| 10  | 5   | 2+2+2+2+2                  |
| 12  | 2   | 5+7                        |
| 12  | 3   | 2+3+7                      |
| 12  | 3   | 2+5+5                      |
| 12  | 4   | 2+2+3+5                    |
| 12  | 4   | 3+3+3+3                    |
| 12  | 6   | 2+2+2+2+2+2                |
| 14  | 2   | 3+11                       |
| 14  | 2   | 7+7                        |
| 14  | 7   | 2+2+2+2+2+2+2              |
| 15  | 3   | 2+2+11                     |
| 15  | 3   | 3+5+7                      |
| 15  | 3   | 5+5+5                      |
| 15  | 5   | 2+2+2+2+7                  |
| 15  | 5   | 2+2+3+3+5                  |
| 15  | 5   | 3+3+3+3+3                  |
| 16  | 2   | 3+13                       |
| 16  | 2   | 5+11                       |
| 16  | 4   | 2+2+5+7                    |
| 16  | 4   | 3+3+3+7                    |
| 16  | 4   | 3+3+5+5                    |
| 16  | 8   | 2+2+2+2+2+2+2+2            |
| 18  | 2   | 5+13                       |
| 18  | 2   | 7+11                       |
| 18  | 3   | 2+3+13                     |
| 18  | 3   | 2+5+11                     |
| 18  | 6   | 2+2+2+2+3+7                |
| 18  | 6   | 2+2+2+2+5+5                |
| 18  | 6   | 2+2+3+3+3+5                |
| 18  | 6   | 3+3+3+3+3+3                |
| 18  | 9   | 2+2+2+2+2+2+2+2+2          |
| 20  | 2   | 3+17                       |
| 20  | 2   | 7+13                       |
| 20  | 4   | 2+2+3+13                   |
| 20  | 4   | 2+2+5+11                   |

|    |    |                       |
|----|----|-----------------------|
| 20 | 4  | 3+3+3+11              |
| 20 | 4  | 3+3+7+7               |
| 20 | 4  | 3+5+5+7               |
| 20 | 4  | 5+5+5+5               |
| 20 | 5  | 2+2+2+3+11            |
| 20 | 5  | 2+2+2+7+7             |
| 20 | 5  | 2+3+3+5+7             |
| 20 | 5  | 2+3+5+5+5             |
| 20 | 10 | 2+2+2+2+2+2+2+2+2     |
| 21 | 3  | 2+2+17                |
| 21 | 3  | 3+5+13                |
| 21 | 3  | 3+7+11                |
| 21 | 3  | 5+5+11                |
| 21 | 3  | 7+7+7                 |
| 21 | 7  | 2+2+2+2+3+3+7         |
| 21 | 7  | 2+2+2+2+3+5+5         |
| 21 | 7  | 2+2+3+3+3+3+5         |
| 21 | 7  | 3+3+3+3+3+3+3         |
| 22 | 2  | 3+19                  |
| 22 | 2  | 5+17                  |
| 22 | 2  | 11+11                 |
| 22 | 11 | 2+2+2+2+2+2+2+2+2+2+2 |
| 24 | 2  | 5+19                  |
| 24 | 2  | 7+17                  |
| 24 | 2  | 11+13                 |
| 24 | 3  | 2+3+19                |
| 24 | 3  | 2+5+17                |
| 24 | 3  | 2+11+11               |
| 24 | 4  | 2+2+3+17              |
| 24 | 4  | 2+2+7+13              |
| 24 | 4  | 3+3+5+13              |
| 24 | 4  | 3+3+7+11              |
| 24 | 4  | 3+5+5+11              |
| 24 | 4  | 3+7+7+7               |
| 24 | 4  | 5+5+7+7               |
| 24 | 6  | 2+2+2+2+3+13          |
| 24 | 6  | 2+2+2+2+5+11          |
| 24 | 6  | 2+2+3+3+3+11          |
| 24 | 6  | 2+2+3+3+7+7           |
| 24 | 6  | 2+2+3+5+5+7           |
| 24 | 6  | 2+2+5+5+5+5           |
| 24 | 6  | 3+3+3+3+5+7           |
| 24 | 6  | 3+3+3+5+5+5           |
| 24 | 8  | 2+2+2+2+2+2+5+7       |
| 24 | 8  | 2+2+2+2+3+3+3+7       |
| 24 | 8  | 2+2+2+2+3+3+5+5       |
| 24 | 8  | 2+2+3+3+3+3+3+5       |

|    |    |                         |
|----|----|-------------------------|
| 24 | 8  | 3+3+3+3+3+3+3           |
| 24 | 12 | 2+2+2+2+2+2+2+2+2+2+2   |
| 25 | 5  | 2+2+2+2+17              |
| 25 | 5  | 2+2+3+5+13              |
| 25 | 5  | 2+2+3+7+11              |
| 25 | 5  | 2+2+5+5+11              |
| 25 | 5  | 2+2+7+7+7               |
| 25 | 5  | 3+3+3+3+13              |
| 25 | 5  | 3+3+3+5+11              |
| 25 | 5  | 3+3+5+7+7               |
| 25 | 5  | 3+5+5+5+7               |
| 25 | 5  | 5+5+5+5+5               |
| 26 | 2  | 3+23                    |
| 26 | 2  | 7+19                    |
| 26 | 2  | 13+13                   |
| 26 | 13 | 2+2+2+2+2+2+2+2+2+2+2+2 |
| 27 | 3  | 2+2+23                  |
| 27 | 3  | 3+5+19                  |
| 27 | 3  | 3+7+17                  |
| 27 | 3  | 3+11+13                 |
| 27 | 3  | 5+5+17                  |
| 27 | 3  | 5+11+11                 |
| 27 | 3  | 7+7+13                  |
| 27 | 9  | 2+2+2+2+2+2+2+2+11      |
| 27 | 9  | 2+2+2+2+2+2+3+5+7       |
| 27 | 9  | 2+2+2+2+2+2+5+5+5       |
| 27 | 9  | 2+2+2+2+3+3+3+3+7       |
| 27 | 9  | 2+2+2+2+3+3+3+5+5       |
| 27 | 9  | 2+2+3+3+3+3+3+3+5       |
| 27 | 9  | 3+3+3+3+3+3+3+3+3       |
| 28 | 2  | 5+23                    |
| 28 | 2  | 11+17                   |
| 28 | 4  | 2+2+5+19                |
| 28 | 4  | 2+2+7+17                |
| 28 | 4  | 2+2+11+13               |
| 28 | 4  | 3+3+3+19                |
| 28 | 4  | 3+3+5+17                |
| 28 | 4  | 3+3+11+11               |
| 28 | 4  | 3+5+7+13                |
| 28 | 4  | 3+7+7+11                |
| 28 | 4  | 5+5+5+13                |
| 28 | 4  | 5+5+7+11                |
| 28 | 4  | 7+7+7+7                 |
| 28 | 7  | 2+2+2+2+2+5+13          |
| 28 | 7  | 2+2+2+2+2+7+11          |
| 28 | 7  | 2+2+2+3+3+3+13          |
| 28 | 7  | 2+2+2+3+3+5+11          |

|    |    |                         |
|----|----|-------------------------|
| 28 | 7  | 2+2+2+3+5+7+7           |
| 28 | 7  | 2+2+2+5+5+5+7           |
| 28 | 7  | 2+3+3+3+3+3+11          |
| 28 | 7  | 2+3+3+3+3+7+7           |
| 28 | 7  | 2+3+3+3+5+5+7           |
| 28 | 7  | 2+3+3+5+5+5+5           |
| 28 | 14 | 2+2+2+2+2+2+2+2+2+2+2+2 |
| 30 | 2  | 7+23                    |
| 30 | 2  | 11+19                   |
| 30 | 2  | 13+17                   |
| 30 | 3  | 2+5+23                  |
| 30 | 3  | 2+11+17                 |
| 30 | 5  | 2+2+2+5+19              |
| 30 | 5  | 2+2+2+7+17              |
| 30 | 5  | 2+2+2+11+13             |
| 30 | 5  | 2+3+3+3+19              |
| 30 | 5  | 2+3+3+5+17              |
| 30 | 5  | 2+3+3+11+11             |
| 30 | 5  | 2+3+5+7+13              |
| 30 | 5  | 2+3+7+7+11              |
| 30 | 5  | 2+5+5+5+13              |
| 30 | 5  | 2+5+5+7+11              |
| 30 | 5  | 2+7+7+7+7               |
| 30 | 6  | 2+2+2+2+3+19            |
| 30 | 6  | 2+2+2+2+5+17            |
| 30 | 6  | 2+2+2+2+11+11           |
| 30 | 6  | 2+2+3+3+3+17            |
| 30 | 6  | 2+2+3+3+7+13            |
| 30 | 6  | 2+2+3+5+5+13            |
| 30 | 6  | 2+2+3+5+7+11            |
| 30 | 6  | 2+2+5+5+5+11            |
| 30 | 6  | 2+2+5+7+7+7             |
| 30 | 6  | 3+3+3+3+5+13            |
| 30 | 6  | 3+3+3+3+7+11            |
| 30 | 6  | 3+3+3+5+5+11            |
| 30 | 6  | 3+3+3+7+7+7             |
| 30 | 6  | 3+3+5+5+7+7             |
| 30 | 6  | 3+5+5+5+5+7             |
| 30 | 6  | 5+5+5+5+5+5             |
| 30 | 10 | 2+2+2+2+2+2+2+2+3+11    |
| 30 | 10 | 2+2+2+2+2+2+2+2+7+7     |
| 30 | 10 | 2+2+2+2+2+2+3+3+5+7     |
| 30 | 10 | 2+2+2+2+2+2+3+5+5+5     |
| 30 | 10 | 2+2+2+2+3+3+3+3+3+7     |
| 30 | 10 | 2+2+2+2+3+3+3+3+5+5     |
| 30 | 10 | 2+2+3+3+3+3+3+3+3+5     |
| 30 | 10 | 3+3+3+3+3+3+3+3+3+3     |

|    |    |                               |
|----|----|-------------------------------|
| 30 | 15 | 2+2+2+2+2+2+2+2+2+2+2+2+2+2+2 |
| 32 | 2  | 3+29                          |
| 32 | 2  | 13+19                         |
| 32 | 4  | 2+2+5+23                      |
| 32 | 4  | 2+2+11+17                     |
| 32 | 4  | 3+3+3+23                      |
| 32 | 4  | 3+3+7+19                      |
| 32 | 4  | 3+3+13+13                     |
| 32 | 4  | 3+5+5+19                      |
| 32 | 4  | 3+5+7+17                      |
| 32 | 4  | 3+5+11+13                     |
| 32 | 4  | 3+7+11+11                     |
| 32 | 4  | 5+5+5+17                      |
| 32 | 4  | 5+5+11+11                     |
| 32 | 4  | 5+7+7+13                      |
| 32 | 4  | 7+7+7+11                      |
| 32 | 8  | 2+2+2+2+2+2+3+17              |
| 32 | 8  | 2+2+2+2+2+2+7+13              |
| 32 | 8  | 2+2+2+2+3+3+5+13              |
| 32 | 8  | 2+2+2+2+3+3+7+11              |
| 32 | 8  | 2+2+2+2+3+5+5+11              |
| 32 | 8  | 2+2+2+2+3+7+7+7               |
| 32 | 8  | 2+2+2+2+5+5+7+7               |
| 32 | 8  | 2+2+3+3+3+3+3+13              |
| 32 | 8  | 2+2+3+3+3+3+5+11              |
| 32 | 8  | 2+2+3+3+3+5+7+7               |
| 32 | 8  | 2+2+3+3+5+5+5+7               |
| 32 | 8  | 2+2+3+5+5+5+5+5               |
| 32 | 8  | 3+3+3+3+3+3+3+11              |
| 32 | 8  | 3+3+3+3+3+3+7+7               |
| 32 | 8  | 3+3+3+3+3+5+5+7               |
| 32 | 8  | 3+3+3+3+5+5+5+5               |
| 32 | 16 | 2+2+2+2+2+2+2+2+2+2+2+2+2+2+2 |
| 33 | 3  | 2+2+29                        |
| 33 | 3  | 3+7+23                        |
| 33 | 3  | 3+11+19                       |
| 33 | 3  | 3+13+17                       |
| 33 | 3  | 5+5+23                        |
| 33 | 3  | 5+11+17                       |
| 33 | 3  | 7+7+19                        |
| 33 | 3  | 7+13+13                       |
| 33 | 3  | 11+11+11                      |
| 33 | 11 | 2+2+2+2+2+2+2+2+2+13          |
| 33 | 11 | 2+2+2+2+2+2+2+2+3+3+11        |
| 33 | 11 | 2+2+2+2+2+2+2+2+3+7+7         |
| 33 | 11 | 2+2+2+2+2+2+2+2+5+5+7         |
| 33 | 11 | 2+2+2+2+2+2+3+3+5+7           |

|    |    |                               |
|----|----|-------------------------------|
| 33 | 11 | 2+2+2+2+2+2+3+3+5+5+5         |
| 33 | 11 | 2+2+2+2+3+3+3+3+3+3+7         |
| 33 | 11 | 2+2+2+2+3+3+3+3+3+5+5         |
| 33 | 11 | 2+2+3+3+3+3+3+3+3+3+5         |
| 33 | 11 | 3+3+3+3+3+3+3+3+3+3+3         |
| 34 | 2  | 3+31                          |
| 34 | 2  | 5+29                          |
| 34 | 2  | 11+23                         |
| 34 | 2  | 17+17                         |
| 34 | 17 | 2+2+2+2+2+2+2+2+2+2+2+2+2+2+2 |
| 35 | 5  | 2+2+3+5+23                    |
| 35 | 5  | 2+2+3+11+17                   |
| 35 | 5  | 2+2+5+7+19                    |
| 35 | 5  | 2+2+5+13+13                   |
| 35 | 5  | 2+2+7+7+17                    |
| 35 | 5  | 2+2+7+11+13                   |
| 35 | 5  | 3+3+3+3+23                    |
| 35 | 5  | 3+3+3+7+19                    |
| 35 | 5  | 3+3+3+13+13                   |
| 35 | 5  | 3+3+5+5+19                    |
| 35 | 5  | 3+3+5+7+17                    |
| 35 | 5  | 3+3+5+11+13                   |
| 35 | 5  | 3+3+7+11+11                   |
| 35 | 5  | 3+5+5+5+17                    |
| 35 | 5  | 3+5+5+11+11                   |
| 35 | 5  | 3+5+7+7+13                    |
| 35 | 5  | 3+7+7+7+11                    |
| 35 | 5  | 5+5+5+7+13                    |
| 35 | 5  | 5+5+7+7+11                    |
| 35 | 5  | 7+7+7+7+7                     |
| 35 | 7  | 2+2+2+2+2+2+23                |
| 35 | 7  | 2+2+2+2+3+5+19                |
| 35 | 7  | 2+2+2+2+3+7+17                |
| 35 | 7  | 2+2+2+2+3+11+13               |
| 35 | 7  | 2+2+2+2+5+5+17                |
| 35 | 7  | 2+2+2+2+5+11+11               |
| 35 | 7  | 2+2+2+2+7+7+13                |
| 35 | 7  | 2+2+3+3+3+3+19                |
| 35 | 7  | 2+2+3+3+3+5+17                |
| 35 | 7  | 2+2+3+3+3+11+11               |
| 35 | 7  | 2+2+3+3+5+7+13                |
| 35 | 7  | 2+2+3+3+7+7+11                |
| 35 | 7  | 2+2+3+5+5+5+13                |
| 35 | 7  | 2+2+3+5+5+7+11                |
| 35 | 7  | 2+2+3+7+7+7+7                 |
| 35 | 7  | 2+2+5+5+5+5+11                |
| 35 | 7  | 2+2+5+5+7+7+7                 |

|    |   |                |
|----|---|----------------|
| 35 | 7 | 3+3+3+3+3+3+17 |
| 35 | 7 | 3+3+3+3+3+7+13 |
| 35 | 7 | 3+3+3+3+5+5+13 |
| 35 | 7 | 3+3+3+3+5+7+11 |
| 35 | 7 | 3+3+3+5+5+5+11 |
| 35 | 7 | 3+3+3+5+7+7+7  |
| 35 | 7 | 3+3+5+5+5+7+7  |
| 35 | 7 | 3+5+5+5+5+5+7  |
| 35 | 7 | 5+5+5+5+5+5+5  |
| 36 | 2 | 5+31           |
| 36 | 2 | 7+29           |
| 36 | 2 | 13+23          |
| 36 | 2 | 17+19          |
| 36 | 3 | 2+3+31         |
| 36 | 3 | 2+5+29         |
| 36 | 3 | 2+11+23        |
| 36 | 3 | 2+17+17        |
| 36 | 4 | 2+2+3+29       |
| 36 | 4 | 2+2+13+19      |
| 36 | 4 | 3+3+7+23       |
| 36 | 4 | 3+3+11+19      |
| 36 | 4 | 3+3+13+17      |
| 36 | 4 | 3+5+5+23       |
| 36 | 4 | 3+5+11+17      |
| 36 | 4 | 3+7+7+19       |
| 36 | 4 | 3+7+13+13      |
| 36 | 4 | 3+11+11+11     |
| 36 | 4 | 5+5+7+19       |
| 36 | 4 | 5+5+13+13      |
| 36 | 4 | 5+7+7+17       |
| 36 | 4 | 5+7+11+13      |
| 36 | 4 | 7+7+11+11      |
| 36 | 6 | 2+2+2+2+5+23   |
| 36 | 6 | 2+2+2+2+11+17  |
| 36 | 6 | 2+2+3+3+3+23   |
| 36 | 6 | 2+2+3+3+7+19   |
| 36 | 6 | 2+2+3+3+13+13  |
| 36 | 6 | 2+2+3+5+5+19   |
| 36 | 6 | 2+2+3+5+7+17   |
| 36 | 6 | 2+2+3+5+11+13  |
| 36 | 6 | 2+2+3+7+11+11  |
| 36 | 6 | 2+2+5+5+5+17   |
| 36 | 6 | 2+2+5+5+11+11  |
| 36 | 6 | 2+2+5+7+7+13   |
| 36 | 6 | 2+2+7+7+7+11   |
| 36 | 6 | 3+3+3+3+5+19   |
| 36 | 6 | 3+3+3+3+7+17   |

|    |    |                                   |
|----|----|-----------------------------------|
| 36 | 6  | 3+3+3+3+11+13                     |
| 36 | 6  | 3+3+3+5+5+17                      |
| 36 | 6  | 3+3+3+5+11+11                     |
| 36 | 6  | 3+3+3+7+7+13                      |
| 36 | 6  | 3+3+5+5+7+13                      |
| 36 | 6  | 3+3+5+7+7+11                      |
| 36 | 6  | 3+5+5+5+5+13                      |
| 36 | 6  | 3+5+5+5+7+11                      |
| 36 | 6  | 3+5+7+7+7+7                       |
| 36 | 6  | 5+5+5+5+5+11                      |
| 36 | 6  | 5+5+5+7+7+7                       |
| 36 | 9  | 2+2+2+2+2+2+3+19                  |
| 36 | 9  | 2+2+2+2+2+2+5+17                  |
| 36 | 9  | 2+2+2+2+2+2+11+11                 |
| 36 | 9  | 2+2+2+2+2+3+3+17                  |
| 36 | 9  | 2+2+2+2+2+3+7+13                  |
| 36 | 9  | 2+2+2+2+2+3+5+13                  |
| 36 | 9  | 2+2+2+2+2+3+5+7+11                |
| 36 | 9  | 2+2+2+2+2+5+5+11                  |
| 36 | 9  | 2+2+2+2+2+5+7+7                   |
| 36 | 9  | 2+2+2+3+3+3+3+5+13                |
| 36 | 9  | 2+2+2+3+3+3+3+7+11                |
| 36 | 9  | 2+2+2+3+3+3+5+5+11                |
| 36 | 9  | 2+2+2+3+3+3+7+7                   |
| 36 | 9  | 2+2+2+3+3+5+5+7                   |
| 36 | 9  | 2+2+2+3+5+5+5+5+7                 |
| 36 | 9  | 2+2+2+5+5+5+5+5+5                 |
| 36 | 9  | 2+3+3+3+3+3+3+3+13                |
| 36 | 9  | 2+3+3+3+3+3+3+5+11                |
| 36 | 9  | 2+3+3+3+3+3+5+7                   |
| 36 | 9  | 2+3+3+3+3+5+5+5+7                 |
| 36 | 9  | 2+3+3+3+5+5+5+5+5                 |
| 36 | 12 | 2+2+2+2+2+2+2+2+2+3+13            |
| 36 | 12 | 2+2+2+2+2+2+2+2+2+5+11            |
| 36 | 12 | 2+2+2+2+2+2+2+2+3+3+11            |
| 36 | 12 | 2+2+2+2+2+2+2+2+3+3+7             |
| 36 | 12 | 2+2+2+2+2+2+2+2+3+5+5+7           |
| 36 | 12 | 2+2+2+2+2+2+2+2+5+5+5+5           |
| 36 | 12 | 2+2+2+2+2+2+2+3+3+3+5+7           |
| 36 | 12 | 2+2+2+2+2+2+2+3+3+3+5+5+5         |
| 36 | 12 | 2+2+2+2+3+3+3+3+3+3+3+7           |
| 36 | 12 | 2+2+2+2+3+3+3+3+3+3+5+5           |
| 36 | 12 | 2+2+3+3+3+3+3+3+3+3+3+5           |
| 36 | 12 | 3+3+3+3+3+3+3+3+3+3+3+3           |
| 36 | 18 | 2+2+2+2+2+2+2+2+2+2+2+2+2+2+2+2+2 |
| 38 | 2  | 7+31                              |
| 38 | 2  | 19+19                             |

|    |    |                                   |
|----|----|-----------------------------------|
| 38 | 19 | 2+2+2+2+2+2+2+2+2+2+2+2+2+2+2+2+2 |
| 39 | 3  | 3+5+31                            |
| 39 | 3  | 3+7+29                            |
| 39 | 3  | 3+13+23                           |
| 39 | 3  | 3+17+19                           |
| 39 | 3  | 5+5+29                            |
| 39 | 3  | 5+11+23                           |
| 39 | 3  | 5+17+17                           |
| 39 | 3  | 7+13+19                           |
| 39 | 3  | 11+11+17                          |
| 39 | 3  | 13+13+13                          |
| 39 | 13 | 2+2+2+2+2+2+2+2+2+2+3+3+13        |
| 39 | 13 | 2+2+2+2+2+2+2+2+2+2+3+5+11        |
| 39 | 13 | 2+2+2+2+2+2+2+2+2+2+5+7+7         |
| 39 | 13 | 2+2+2+2+2+2+2+2+3+3+3+3+11        |
| 39 | 13 | 2+2+2+2+2+2+2+2+3+3+3+7+7         |
| 39 | 13 | 2+2+2+2+2+2+2+2+3+3+5+5+7         |
| 39 | 13 | 2+2+2+2+2+2+2+2+3+5+5+5+5         |
| 39 | 13 | 2+2+2+2+2+2+3+3+3+3+3+5+7         |
| 39 | 13 | 2+2+2+2+2+2+3+3+3+3+5+5+5         |
| 39 | 13 | 2+2+2+2+2+2+3+3+3+3+5+5+5         |
| 39 | 13 | 2+2+2+2+3+3+3+3+3+3+3+3+7         |
| 39 | 13 | 2+2+2+2+3+3+3+3+3+3+3+5+5         |
| 39 | 13 | 2+2+3+3+3+3+3+3+3+3+3+3+5         |
| 39 | 13 | 3+3+3+3+3+3+3+3+3+3+3+3+3         |
| 40 | 2  | 3+37                              |
| 40 | 2  | 11+29                             |
| 40 | 2  | 17+23                             |
| 40 | 4  | 2+2+5+31                          |
| 40 | 4  | 2+2+7+29                          |
| 40 | 4  | 2+2+13+23                         |
| 40 | 4  | 2+2+17+19                         |
| 40 | 4  | 3+3+3+31                          |
| 40 | 4  | 3+3+5+29                          |
| 40 | 4  | 3+3+11+23                         |
| 40 | 4  | 3+3+17+17                         |
| 40 | 4  | 3+5+13+19                         |
| 40 | 4  | 3+7+7+23                          |
| 40 | 4  | 3+7+11+19                         |
| 40 | 4  | 3+7+13+17                         |
| 40 | 4  | 3+11+13+13                        |
| 40 | 4  | 5+5+7+23                          |
| 40 | 4  | 5+5+11+19                         |
| 40 | 4  | 5+5+13+17                         |
| 40 | 4  | 5+7+11+17                         |
| 40 | 4  | 5+11+11+13                        |
| 40 | 4  | 7+7+7+19                          |
| 40 | 4  | 7+7+13+13                         |

|    |   |                   |
|----|---|-------------------|
| 40 | 4 | 7+11+11+11        |
| 40 | 5 | 2+2+2+3+31        |
| 40 | 5 | 2+2+2+5+29        |
| 40 | 5 | 2+2+2+11+23       |
| 40 | 5 | 2+2+2+17+17       |
| 40 | 5 | 2+3+3+3+29        |
| 40 | 5 | 2+3+3+13+19       |
| 40 | 5 | 2+3+5+7+23        |
| 40 | 5 | 2+3+5+11+19       |
| 40 | 5 | 2+3+5+13+17       |
| 40 | 5 | 2+3+7+11+17       |
| 40 | 5 | 2+3+11+11+13      |
| 40 | 5 | 2+5+5+5+23        |
| 40 | 5 | 2+5+5+11+17       |
| 40 | 5 | 2+5+7+7+19        |
| 40 | 5 | 2+5+7+13+13       |
| 40 | 5 | 2+5+11+11+11      |
| 40 | 5 | 2+7+7+7+17        |
| 40 | 5 | 2+7+7+11+13       |
| 40 | 8 | 2+2+2+2+2+2+5+23  |
| 40 | 8 | 2+2+2+2+2+2+11+17 |
| 40 | 8 | 2+2+2+2+3+3+3+23  |
| 40 | 8 | 2+2+2+2+3+3+7+19  |
| 40 | 8 | 2+2+2+2+3+3+13+13 |
| 40 | 8 | 2+2+2+2+3+5+5+19  |
| 40 | 8 | 2+2+2+2+3+5+7+17  |
| 40 | 8 | 2+2+2+2+3+5+11+13 |
| 40 | 8 | 2+2+2+2+3+7+11+11 |
| 40 | 8 | 2+2+2+2+5+5+5+17  |
| 40 | 8 | 2+2+2+2+5+5+11+11 |
| 40 | 8 | 2+2+2+2+5+7+7+13  |
| 40 | 8 | 2+2+2+2+7+7+7+11  |
| 40 | 8 | 2+2+3+3+3+3+5+19  |
| 40 | 8 | 2+2+3+3+3+3+7+17  |
| 40 | 8 | 2+2+3+3+3+3+11+13 |
| 40 | 8 | 2+2+3+3+3+5+5+17  |
| 40 | 8 | 2+2+3+3+3+5+11+11 |
| 40 | 8 | 2+2+3+3+3+7+7+13  |
| 40 | 8 | 2+2+3+3+5+5+7+13  |
| 40 | 8 | 2+2+3+3+5+7+7+11  |
| 40 | 8 | 2+2+3+5+5+5+5+13  |
| 40 | 8 | 2+2+3+5+5+5+7+11  |
| 40 | 8 | 2+2+3+5+7+7+7+7   |
| 40 | 8 | 2+2+5+5+5+5+5+11  |
| 40 | 8 | 2+2+5+5+5+7+7+7   |
| 40 | 8 | 3+3+3+3+3+3+3+19  |
| 40 | 8 | 3+3+3+3+3+3+5+17  |

|    |    |                                   |
|----|----|-----------------------------------|
| 40 | 8  | 3+3+3+3+3+11+11                   |
| 40 | 8  | 3+3+3+3+3+5+7+13                  |
| 40 | 8  | 3+3+3+3+3+7+7+11                  |
| 40 | 8  | 3+3+3+3+5+5+5+13                  |
| 40 | 8  | 3+3+3+3+5+5+7+11                  |
| 40 | 8  | 3+3+3+3+7+7+7+7                   |
| 40 | 8  | 3+3+3+5+5+5+5+11                  |
| 40 | 8  | 3+3+3+5+5+7+7+7                   |
| 40 | 8  | 3+3+5+5+5+5+7+7                   |
| 40 | 8  | 3+5+5+5+5+5+5+7                   |
| 40 | 8  | 5+5+5+5+5+5+5+5                   |
| 40 | 10 | 2+2+2+2+2+2+2+5+19                |
| 40 | 10 | 2+2+2+2+2+2+2+7+17                |
| 40 | 10 | 2+2+2+2+2+2+2+11+13               |
| 40 | 10 | 2+2+2+2+2+3+3+19                  |
| 40 | 10 | 2+2+2+2+2+3+3+5+17                |
| 40 | 10 | 2+2+2+2+2+3+3+11+11               |
| 40 | 10 | 2+2+2+2+2+3+5+7+13                |
| 40 | 10 | 2+2+2+2+2+3+7+7+11                |
| 40 | 10 | 2+2+2+2+2+5+5+5+13                |
| 40 | 10 | 2+2+2+2+2+5+5+7+11                |
| 40 | 10 | 2+2+2+2+2+7+7+7+7                 |
| 40 | 10 | 2+2+2+2+3+3+3+3+17                |
| 40 | 10 | 2+2+2+2+3+3+3+3+7+13              |
| 40 | 10 | 2+2+2+2+3+3+3+5+5+13              |
| 40 | 10 | 2+2+2+2+3+3+3+5+7+11              |
| 40 | 10 | 2+2+2+2+3+3+5+5+5+11              |
| 40 | 10 | 2+2+2+2+3+3+5+7+7+7               |
| 40 | 10 | 2+2+2+2+3+5+5+5+7+7               |
| 40 | 10 | 2+2+2+2+5+5+5+5+5+7               |
| 40 | 10 | 2+2+3+3+3+3+3+3+5+13              |
| 40 | 10 | 2+2+3+3+3+3+3+3+7+11              |
| 40 | 10 | 2+2+3+3+3+3+3+5+5+11              |
| 40 | 10 | 2+2+3+3+3+3+3+7+7+7               |
| 40 | 10 | 2+2+3+3+3+3+5+5+7+7               |
| 40 | 10 | 2+2+3+3+3+5+5+5+5+7               |
| 40 | 10 | 2+2+3+3+5+5+5+5+5+5               |
| 40 | 10 | 3+3+3+3+3+3+3+3+13                |
| 40 | 10 | 3+3+3+3+3+3+3+5+11                |
| 40 | 10 | 3+3+3+3+3+3+5+7+7                 |
| 40 | 10 | 3+3+3+3+3+5+5+5+7                 |
| 40 | 10 | 3+3+3+3+5+5+5+5+5                 |
| 40 | 20 | 2+2+2+2+2+2+2+2+2+2+2+2+2+2+2+2+2 |
| 42 | 2  | 5+37                              |
| 42 | 2  | 11+31                             |
| 42 | 2  | 13+29                             |

|    |   |                |
|----|---|----------------|
| 42 | 2 | 19+23          |
| 42 | 3 | 2+3+37         |
| 42 | 3 | 2+11+29        |
| 42 | 3 | 2+17+23        |
| 42 | 6 | 2+2+2+2+3+31   |
| 42 | 6 | 2+2+2+2+5+29   |
| 42 | 6 | 2+2+2+2+11+23  |
| 42 | 6 | 2+2+2+2+17+17  |
| 42 | 6 | 2+2+3+3+3+29   |
| 42 | 6 | 2+2+3+3+13+19  |
| 42 | 6 | 2+2+3+5+7+23   |
| 42 | 6 | 2+2+3+5+11+19  |
| 42 | 6 | 2+2+3+5+13+17  |
| 42 | 6 | 2+2+3+7+11+17  |
| 42 | 6 | 2+2+3+11+11+13 |
| 42 | 6 | 2+2+5+5+5+23   |
| 42 | 6 | 2+2+5+5+11+17  |
| 42 | 6 | 2+2+5+7+7+19   |
| 42 | 6 | 2+2+5+7+13+13  |
| 42 | 6 | 2+2+5+11+11+11 |
| 42 | 6 | 2+2+7+7+7+17   |
| 42 | 6 | 2+2+7+7+11+13  |
| 42 | 6 | 3+3+3+3+7+23   |
| 42 | 6 | 3+3+3+3+11+19  |
| 42 | 6 | 3+3+3+3+13+17  |
| 42 | 6 | 3+3+3+5+5+23   |
| 42 | 6 | 3+3+3+5+11+17  |
| 42 | 6 | 3+3+3+7+7+19   |
| 42 | 6 | 3+3+3+7+13+13  |
| 42 | 6 | 3+3+3+11+11+11 |
| 42 | 6 | 3+3+5+5+7+19   |
| 42 | 6 | 3+3+5+5+13+13  |
| 42 | 6 | 3+3+5+7+7+17   |
| 42 | 6 | 3+3+5+7+11+13  |
| 42 | 6 | 3+3+7+7+11+11  |
| 42 | 6 | 3+5+5+5+5+19   |
| 42 | 6 | 3+5+5+5+7+17   |
| 42 | 6 | 3+5+5+5+11+13  |
| 42 | 6 | 3+5+5+7+11+11  |
| 42 | 6 | 3+5+7+7+7+13   |
| 42 | 6 | 3+7+7+7+7+11   |
| 42 | 6 | 5+5+5+5+5+17   |
| 42 | 6 | 5+5+5+5+11+11  |
| 42 | 6 | 5+5+5+7+7+13   |
| 42 | 6 | 5+5+7+7+7+11   |
| 42 | 6 | 7+7+7+7+7+7    |
| 42 | 7 | 2+2+2+2+2+3+29 |

|    |    |                             |
|----|----|-----------------------------|
| 42 | 7  | 2+2+2+2+2+13+19             |
| 42 | 7  | 2+2+2+3+3+7+23              |
| 42 | 7  | 2+2+2+3+3+11+19             |
| 42 | 7  | 2+2+2+3+3+13+17             |
| 42 | 7  | 2+2+2+3+5+5+23              |
| 42 | 7  | 2+2+2+3+5+11+17             |
| 42 | 7  | 2+2+2+3+7+7+19              |
| 42 | 7  | 2+2+2+3+7+13+13             |
| 42 | 7  | 2+2+2+3+11+11+11            |
| 42 | 7  | 2+2+2+5+5+7+19              |
| 42 | 7  | 2+2+2+5+5+13+13             |
| 42 | 7  | 2+2+2+5+7+7+17              |
| 42 | 7  | 2+2+2+5+7+11+13             |
| 42 | 7  | 2+2+2+7+7+11+11             |
| 42 | 7  | 2+3+3+3+3+5+23              |
| 42 | 7  | 2+3+3+3+3+11+17             |
| 42 | 7  | 2+3+3+3+5+7+19              |
| 42 | 7  | 2+3+3+3+5+13+13             |
| 42 | 7  | 2+3+3+3+7+7+17              |
| 42 | 7  | 2+3+3+3+7+11+13             |
| 42 | 7  | 2+3+3+5+5+5+19              |
| 42 | 7  | 2+3+3+5+5+7+17              |
| 42 | 7  | 2+3+3+5+5+11+13             |
| 42 | 7  | 2+3+3+5+7+11+11             |
| 42 | 7  | 2+3+3+7+7+7+13              |
| 42 | 7  | 2+3+5+5+5+5+17              |
| 42 | 7  | 2+3+5+5+5+11+11             |
| 42 | 7  | 2+3+5+5+7+7+13              |
| 42 | 7  | 2+3+5+7+7+7+11              |
| 42 | 7  | 2+5+5+5+5+7+13              |
| 42 | 7  | 2+5+5+5+7+7+11              |
| 42 | 7  | 2+5+7+7+7+7+7               |
| 42 | 14 | 2+2+2+2+2+2+2+2+2+2+5+13    |
| 42 | 14 | 2+2+2+2+2+2+2+2+2+2+7+11    |
| 42 | 14 | 2+2+2+2+2+2+2+2+2+3+3+13    |
| 42 | 14 | 2+2+2+2+2+2+2+2+2+3+3+5+11  |
| 42 | 14 | 2+2+2+2+2+2+2+2+2+3+5+7+7   |
| 42 | 14 | 2+2+2+2+2+2+2+2+2+5+5+5+7   |
| 42 | 14 | 2+2+2+2+2+2+2+2+3+3+3+3+11  |
| 42 | 14 | 2+2+2+2+2+2+2+2+3+3+3+3+7+7 |
| 42 | 14 | 2+2+2+2+2+2+2+2+3+3+3+5+5+7 |
| 42 | 14 | 2+2+2+2+2+2+2+2+3+3+5+5+5+5 |
| 42 | 14 | 2+2+2+2+2+2+3+3+3+3+3+3+5+7 |
| 42 | 14 | 2+2+2+2+2+2+3+3+3+3+3+5+5+5 |
| 42 | 14 | 2+2+2+2+3+3+3+3+3+3+3+3+7   |
| 42 | 14 | 2+2+2+2+3+3+3+3+3+3+3+3+5+5 |
| 42 | 14 | 2+2+3+3+3+3+3+3+3+3+3+3+3+5 |

|    |    |                                     |
|----|----|-------------------------------------|
| 42 | 14 | 3+3+3+3+3+3+3+3+3+3+3+3+3           |
| 42 | 21 | 2+2+2+2+2+2+2+2+2+2+2+2+2+2+2+2+2+2 |
| 44 | 2  | 3+41                                |
| 44 | 2  | 7+37                                |
| 44 | 2  | 13+31                               |
| 44 | 4  | 2+2+3+37                            |
| 44 | 4  | 2+2+11+29                           |
| 44 | 4  | 2+2+17+23                           |
| 44 | 4  | 3+3+7+31                            |
| 44 | 4  | 3+3+19+19                           |
| 44 | 4  | 3+5+5+31                            |
| 44 | 4  | 3+5+7+29                            |
| 44 | 4  | 3+5+13+23                           |
| 44 | 4  | 3+5+17+19                           |
| 44 | 4  | 3+7+11+23                           |
| 44 | 4  | 3+7+17+17                           |
| 44 | 4  | 3+11+11+19                          |
| 44 | 4  | 3+11+13+17                          |
| 44 | 4  | 5+5+5+29                            |
| 44 | 4  | 5+5+11+23                           |
| 44 | 4  | 5+5+17+17                           |
| 44 | 4  | 5+7+13+19                           |
| 44 | 4  | 5+11+11+17                          |
| 44 | 4  | 5+13+13+13                          |
| 44 | 4  | 7+7+7+23                            |
| 44 | 4  | 7+7+11+19                           |
| 44 | 4  | 7+7+13+17                           |
| 44 | 4  | 7+11+13+13                          |
| 44 | 4  | 11+11+11+11                         |
| 44 | 11 | 2+2+2+2+2+2+2+2+2+3+23              |
| 44 | 11 | 2+2+2+2+2+2+2+2+2+7+19              |
| 44 | 11 | 2+2+2+2+2+2+2+2+2+13+13             |
| 44 | 11 | 2+2+2+2+2+2+2+2+3+3+5+19            |
| 44 | 11 | 2+2+2+2+2+2+2+2+3+3+7+17            |
| 44 | 11 | 2+2+2+2+2+2+2+2+3+3+11+13           |
| 44 | 11 | 2+2+2+2+2+2+2+2+3+5+5+17            |
| 44 | 11 | 2+2+2+2+2+2+2+2+3+5+11+11           |
| 44 | 11 | 2+2+2+2+2+2+2+2+3+7+7+13            |
| 44 | 11 | 2+2+2+2+2+2+2+2+5+5+7+13            |
| 44 | 11 | 2+2+2+2+2+2+2+2+5+7+7+11            |
| 44 | 11 | 2+2+2+2+2+3+3+3+3+3+19              |
| 44 | 11 | 2+2+2+2+2+3+3+3+3+5+17              |
| 44 | 11 | 2+2+2+2+2+3+3+3+3+11+11             |
| 44 | 11 | 2+2+2+2+2+3+3+3+5+7+13              |
| 44 | 11 | 2+2+2+2+2+3+3+3+7+7+11              |
| 44 | 11 | 2+2+2+2+2+3+3+5+5+5+13              |







|    |   |                 |
|----|---|-----------------|
| 48 | 4 | 7+7+11+23       |
| 48 | 4 | 7+7+17+17       |
| 48 | 4 | 7+11+11+19      |
| 48 | 4 | 7+11+13+17      |
| 48 | 4 | 11+11+13+13     |
| 48 | 6 | 2+2+2+2+3+37    |
| 48 | 6 | 2+2+2+2+11+29   |
| 48 | 6 | 2+2+2+2+17+23   |
| 48 | 6 | 2+2+3+3+7+31    |
| 48 | 6 | 2+2+3+3+19+19   |
| 48 | 6 | 2+2+3+5+5+31    |
| 48 | 6 | 2+2+3+5+7+29    |
| 48 | 6 | 2+2+3+5+13+23   |
| 48 | 6 | 2+2+3+5+17+19   |
| 48 | 6 | 2+2+3+7+11+23   |
| 48 | 6 | 2+2+3+7+17+17   |
| 48 | 6 | 2+2+3+11+11+19  |
| 48 | 6 | 2+2+3+11+13+17  |
| 48 | 6 | 2+2+5+5+5+29    |
| 48 | 6 | 2+2+5+5+11+23   |
| 48 | 6 | 2+2+5+5+17+17   |
| 48 | 6 | 2+2+5+7+13+19   |
| 48 | 6 | 2+2+5+11+11+17  |
| 48 | 6 | 2+2+5+13+13+13  |
| 48 | 6 | 2+2+7+7+7+23    |
| 48 | 6 | 2+2+7+7+11+19   |
| 48 | 6 | 2+2+7+7+13+17   |
| 48 | 6 | 2+2+7+11+13+13  |
| 48 | 6 | 2+2+11+11+11+11 |
| 48 | 6 | 3+3+3+3+5+31    |
| 48 | 6 | 3+3+3+3+7+29    |
| 48 | 6 | 3+3+3+3+13+23   |
| 48 | 6 | 3+3+3+3+17+19   |
| 48 | 6 | 3+3+3+5+5+29    |
| 48 | 6 | 3+3+3+5+11+23   |
| 48 | 6 | 3+3+3+5+17+17   |
| 48 | 6 | 3+3+3+7+13+19   |
| 48 | 6 | 3+3+3+11+11+17  |
| 48 | 6 | 3+3+3+13+13+13  |
| 48 | 6 | 3+3+5+5+13+19   |
| 48 | 6 | 3+3+5+7+7+23    |
| 48 | 6 | 3+3+5+7+11+19   |
| 48 | 6 | 3+3+5+7+13+17   |
| 48 | 6 | 3+3+5+11+13+13  |
| 48 | 6 | 3+3+7+7+11+17   |
| 48 | 6 | 3+3+7+11+11+13  |
| 48 | 6 | 3+5+5+5+7+23    |

|    |   |                    |
|----|---|--------------------|
| 48 | 6 | 3+5+5+5+11+19      |
| 48 | 6 | 3+5+5+5+13+17      |
| 48 | 6 | 3+5+5+7+11+17      |
| 48 | 6 | 3+5+5+11+11+13     |
| 48 | 6 | 3+5+7+7+7+19       |
| 48 | 6 | 3+5+7+7+13+13      |
| 48 | 6 | 3+5+7+11+11+11     |
| 48 | 6 | 3+7+7+7+7+17       |
| 48 | 6 | 3+7+7+7+11+13      |
| 48 | 6 | 5+5+5+5+5+23       |
| 48 | 6 | 5+5+5+5+11+17      |
| 48 | 6 | 5+5+5+7+7+19       |
| 48 | 6 | 5+5+5+7+13+13      |
| 48 | 6 | 5+5+5+11+11+11     |
| 48 | 6 | 5+5+7+7+7+17       |
| 48 | 6 | 5+5+7+7+11+13      |
| 48 | 6 | 5+7+7+7+11+11      |
| 48 | 6 | 7+7+7+7+7+13       |
| 48 | 8 | 2+2+2+2+2+2+5+31   |
| 48 | 8 | 2+2+2+2+2+2+7+29   |
| 48 | 8 | 2+2+2+2+2+2+13+23  |
| 48 | 8 | 2+2+2+2+2+2+17+19  |
| 48 | 8 | 2+2+2+2+3+3+3+31   |
| 48 | 8 | 2+2+2+2+3+3+5+29   |
| 48 | 8 | 2+2+2+2+3+3+11+23  |
| 48 | 8 | 2+2+2+2+3+3+17+17  |
| 48 | 8 | 2+2+2+2+3+5+13+19  |
| 48 | 8 | 2+2+2+2+3+7+7+23   |
| 48 | 8 | 2+2+2+2+3+7+11+19  |
| 48 | 8 | 2+2+2+2+3+7+13+17  |
| 48 | 8 | 2+2+2+2+3+11+13+13 |
| 48 | 8 | 2+2+2+2+5+5+7+23   |
| 48 | 8 | 2+2+2+2+5+5+11+19  |
| 48 | 8 | 2+2+2+2+5+5+13+17  |
| 48 | 8 | 2+2+2+2+5+7+11+17  |
| 48 | 8 | 2+2+2+2+5+11+11+13 |
| 48 | 8 | 2+2+2+2+7+7+7+19   |
| 48 | 8 | 2+2+2+2+7+7+13+13  |
| 48 | 8 | 2+2+2+2+7+11+11+11 |
| 48 | 8 | 2+2+3+3+3+3+3+29   |
| 48 | 8 | 2+2+3+3+3+3+13+19  |
| 48 | 8 | 2+2+3+3+3+5+7+23   |
| 48 | 8 | 2+2+3+3+3+5+11+19  |
| 48 | 8 | 2+2+3+3+3+5+13+17  |
| 48 | 8 | 2+2+3+3+3+7+11+17  |
| 48 | 8 | 2+2+3+3+3+11+11+13 |
| 48 | 8 | 2+2+3+3+5+5+5+23   |

|    |   |                    |
|----|---|--------------------|
| 48 | 8 | 2+2+3+3+5+5+11+17  |
| 48 | 8 | 2+2+3+3+5+7+7+19   |
| 48 | 8 | 2+2+3+3+5+7+13+13  |
| 48 | 8 | 2+2+3+3+5+11+11+11 |
| 48 | 8 | 2+2+3+3+7+7+7+17   |
| 48 | 8 | 2+2+3+3+7+7+11+13  |
| 48 | 8 | 2+2+3+5+5+5+7+19   |
| 48 | 8 | 2+2+3+5+5+5+13+13  |
| 48 | 8 | 2+2+3+5+5+7+7+17   |
| 48 | 8 | 2+2+3+5+5+7+11+13  |
| 48 | 8 | 2+2+3+5+7+7+11+11  |
| 48 | 8 | 2+2+3+7+7+7+7+13   |
| 48 | 8 | 2+2+5+5+5+5+5+19   |
| 48 | 8 | 2+2+5+5+5+5+7+17   |
| 48 | 8 | 2+2+5+5+5+5+11+13  |
| 48 | 8 | 2+2+5+5+5+7+11+11  |
| 48 | 8 | 2+2+5+5+7+7+7+13   |
| 48 | 8 | 2+2+5+7+7+7+7+11   |
| 48 | 8 | 3+3+3+3+3+3+7+23   |
| 48 | 8 | 3+3+3+3+3+3+11+19  |
| 48 | 8 | 3+3+3+3+3+3+13+17  |
| 48 | 8 | 3+3+3+3+3+5+5+23   |
| 48 | 8 | 3+3+3+3+3+5+11+17  |
| 48 | 8 | 3+3+3+3+3+7+7+19   |
| 48 | 8 | 3+3+3+3+3+7+13+13  |
| 48 | 8 | 3+3+3+3+3+11+11+11 |
| 48 | 8 | 3+3+3+3+5+5+7+19   |
| 48 | 8 | 3+3+3+3+5+5+13+13  |
| 48 | 8 | 3+3+3+3+5+7+7+17   |
| 48 | 8 | 3+3+3+3+5+7+11+13  |
| 48 | 8 | 3+3+3+3+7+7+11+11  |
| 48 | 8 | 3+3+3+5+5+5+5+19   |
| 48 | 8 | 3+3+3+5+5+5+7+17   |
| 48 | 8 | 3+3+3+5+5+5+11+13  |
| 48 | 8 | 3+3+3+5+5+7+11+11  |
| 48 | 8 | 3+3+3+5+7+7+7+13   |
| 48 | 8 | 3+3+3+7+7+7+7+11   |
| 48 | 8 | 3+3+5+5+5+5+5+17   |
| 48 | 8 | 3+3+5+5+5+5+11+11  |
| 48 | 8 | 3+3+5+5+5+7+7+13   |
| 48 | 8 | 3+3+5+5+7+7+7+7    |
| 48 | 8 | 3+5+5+5+5+5+7+13   |
| 48 | 8 | 3+5+5+5+5+7+7+11   |
| 48 | 8 | 3+5+5+7+7+7+7+7    |
| 48 | 8 | 5+5+5+5+5+5+5+13   |
| 48 | 8 | 5+5+5+5+5+5+7+11   |

|    |    |                           |
|----|----|---------------------------|
| 48 | 8  | 5+5+5+5+7+7+7+7           |
| 48 | 12 | 2+2+2+2+2+2+2+2+2+5+23    |
| 48 | 12 | 2+2+2+2+2+2+2+2+2+11+17   |
| 48 | 12 | 2+2+2+2+2+2+2+2+3+3+3+23  |
| 48 | 12 | 2+2+2+2+2+2+2+2+3+3+7+19  |
| 48 | 12 | 2+2+2+2+2+2+2+2+3+3+13+13 |
| 48 | 12 | 2+2+2+2+2+2+2+2+3+5+5+19  |
| 48 | 12 | 2+2+2+2+2+2+2+2+3+5+7+17  |
| 48 | 12 | 2+2+2+2+2+2+2+2+3+5+11+13 |
| 48 | 12 | 2+2+2+2+2+2+2+2+3+7+11+11 |
| 48 | 12 | 2+2+2+2+2+2+2+2+5+5+5+17  |
| 48 | 12 | 2+2+2+2+2+2+2+2+5+5+11+11 |
| 48 | 12 | 2+2+2+2+2+2+2+2+5+7+7+13  |
| 48 | 12 | 2+2+2+2+2+2+2+2+7+7+7+11  |
| 48 | 12 | 2+2+2+2+2+3+3+3+3+5+19    |
| 48 | 12 | 2+2+2+2+2+3+3+3+3+7+17    |
| 48 | 12 | 2+2+2+2+2+3+3+3+3+11+13   |
| 48 | 12 | 2+2+2+2+2+3+3+3+5+5+17    |
| 48 | 12 | 2+2+2+2+2+3+3+3+5+11+11   |
| 48 | 12 | 2+2+2+2+2+3+3+3+7+7+13    |
| 48 | 12 | 2+2+2+2+2+3+3+5+5+7+13    |
| 48 | 12 | 2+2+2+2+2+3+3+5+7+7+11    |
| 48 | 12 | 2+2+2+2+2+3+5+5+5+5+13    |
| 48 | 12 | 2+2+2+2+2+3+5+5+5+7+11    |
| 48 | 12 | 2+2+2+2+2+3+5+7+7+7+7     |
| 48 | 12 | 2+2+2+2+2+5+5+5+5+5+11    |
| 48 | 12 | 2+2+2+2+2+5+5+5+7+7+7     |
| 48 | 12 | 2+2+2+2+3+3+3+3+3+3+3+19  |
| 48 | 12 | 2+2+2+2+3+3+3+3+3+3+5+17  |
| 48 | 12 | 2+2+2+2+3+3+3+3+3+3+11+11 |
| 48 | 12 | 2+2+2+2+3+3+3+3+3+5+7+13  |
| 48 | 12 | 2+2+2+2+3+3+3+3+3+7+7+11  |
| 48 | 12 | 2+2+2+2+3+3+3+3+5+5+5+13  |
| 48 | 12 | 2+2+2+2+3+3+3+3+5+5+7+11  |
| 48 | 12 | 2+2+2+2+3+3+3+3+7+7+7+7   |
| 48 | 12 | 2+2+2+2+3+3+3+5+5+5+5+11  |
| 48 | 12 | 2+2+2+2+3+3+3+5+5+7+7+7   |
| 48 | 12 | 2+2+2+2+5+5+5+5+5+5+5+5   |
| 48 | 12 | 2+2+3+3+3+3+3+3+3+3+3+17  |
| 48 | 12 | 2+2+3+3+3+3+3+3+3+3+7+13  |
| 48 | 12 | 2+2+3+3+3+3+3+3+3+5+5+13  |
| 48 | 12 | 2+2+3+3+3+3+3+3+3+5+7+11  |
| 48 | 12 | 2+2+3+3+3+3+3+3+5+5+5+11  |
| 48 | 12 | 2+2+3+3+3+3+3+3+5+7+7+7   |
| 48 | 12 | 2+2+3+3+3+3+3+5+5+5+7+7   |



|    |    |                    |
|----|----|--------------------|
| 49 | 7  | 3+3+5+7+7+11+13    |
| 49 | 7  | 3+3+7+7+7+11+11    |
| 49 | 7  | 3+5+5+5+5+7+19     |
| 49 | 7  | 3+5+5+5+5+13+13    |
| 49 | 7  | 3+5+5+5+7+7+17     |
| 49 | 7  | 3+5+5+5+7+11+13    |
| 49 | 7  | 3+5+5+7+7+11+11    |
| 49 | 7  | 3+5+7+7+7+7+13     |
| 49 | 7  | 3+7+7+7+7+7+11     |
| 49 | 7  | 5+5+5+5+5+5+19     |
| 49 | 7  | 5+5+5+5+5+7+17     |
| 49 | 7  | 5+5+5+5+5+11+13    |
| 49 | 7  | 5+5+5+5+7+11+11    |
| 49 | 7  | 5+5+5+7+7+7+13     |
| 49 | 7  | 5+5+7+7+7+7+11     |
| 49 | 7  | 7+7+7+7+7+7+7      |
| 50 | 2  | 3+47               |
| 50 | 2  | 7+43               |
| 50 | 2  | 13+37              |
| 50 | 2  | 19+31              |
| 50 | 5  | 2+2+2+3+41         |
| 50 | 5  | 2+2+2+7+37         |
| 50 | 5  | 2+2+2+13+31        |
| 50 | 5  | 2+3+3+5+37         |
| 50 | 5  | 2+3+3+11+31        |
| 50 | 5  | 2+3+3+13+29        |
| 50 | 5  | 2+3+3+19+23        |
| 50 | 5  | 2+3+5+11+29        |
| 50 | 5  | 2+3+5+17+23        |
| 50 | 5  | 2+3+7+7+31         |
| 50 | 5  | 2+3+7+19+19        |
| 50 | 5  | 2+3+11+11+23       |
| 50 | 5  | 2+3+11+17+17       |
| 50 | 5  | 2+3+13+13+19       |
| 50 | 5  | 2+5+5+7+31         |
| 50 | 5  | 2+5+5+19+19        |
| 50 | 5  | 2+5+7+7+29         |
| 50 | 5  | 2+5+7+13+23        |
| 50 | 5  | 2+5+7+17+19        |
| 50 | 5  | 2+5+11+13+19       |
| 50 | 5  | 2+5+13+13+17       |
| 50 | 5  | 2+7+7+11+23        |
| 50 | 5  | 2+7+7+17+17        |
| 50 | 5  | 2+7+11+11+19       |
| 50 | 5  | 2+7+11+13+17       |
| 50 | 5  | 2+11+11+13+13      |
| 50 | 10 | 2+2+2+2+2+2+2+3+31 |

|    |    |                        |
|----|----|------------------------|
| 50 | 10 | 2+2+2+2+2+2+2+5+29     |
| 50 | 10 | 2+2+2+2+2+2+2+11+23    |
| 50 | 10 | 2+2+2+2+2+2+2+17+17    |
| 50 | 10 | 2+2+2+2+2+2+3+3+29     |
| 50 | 10 | 2+2+2+2+2+2+3+3+13+19  |
| 50 | 10 | 2+2+2+2+2+2+3+5+7+23   |
| 50 | 10 | 2+2+2+2+2+2+3+5+11+19  |
| 50 | 10 | 2+2+2+2+2+2+3+5+13+17  |
| 50 | 10 | 2+2+2+2+2+2+3+7+11+17  |
| 50 | 10 | 2+2+2+2+2+2+3+11+11+13 |
| 50 | 10 | 2+2+2+2+2+2+5+5+5+23   |
| 50 | 10 | 2+2+2+2+2+2+5+5+11+17  |
| 50 | 10 | 2+2+2+2+2+2+5+7+7+19   |
| 50 | 10 | 2+2+2+2+2+2+5+7+13+13  |
| 50 | 10 | 2+2+2+2+2+2+5+11+11+11 |
| 50 | 10 | 2+2+2+2+2+2+7+7+7+17   |
| 50 | 10 | 2+2+2+2+2+2+7+7+11+13  |
| 50 | 10 | 2+2+2+2+3+3+3+3+7+23   |
| 50 | 10 | 2+2+2+2+3+3+3+3+11+19  |
| 50 | 10 | 2+2+2+2+3+3+3+3+13+17  |
| 50 | 10 | 2+2+2+2+3+3+3+5+5+23   |
| 50 | 10 | 2+2+2+2+3+3+3+5+11+17  |
| 50 | 10 | 2+2+2+2+3+3+3+7+7+19   |
| 50 | 10 | 2+2+2+2+3+3+3+7+13+13  |
| 50 | 10 | 2+2+2+2+3+3+3+11+11+11 |
| 50 | 10 | 2+2+2+2+3+3+5+5+7+19   |
| 50 | 10 | 2+2+2+2+3+3+5+5+13+13  |
| 50 | 10 | 2+2+2+2+3+3+5+7+7+17   |
| 50 | 10 | 2+2+2+2+3+3+5+7+11+13  |
| 50 | 10 | 2+2+2+2+3+3+7+7+11+11  |
| 50 | 10 | 2+2+2+2+3+5+5+5+5+19   |
| 50 | 10 | 2+2+2+2+3+5+5+5+7+17   |
| 50 | 10 | 2+2+2+2+3+5+5+5+11+13  |
| 50 | 10 | 2+2+2+2+3+5+5+7+11+11  |
| 50 | 10 | 2+2+2+2+3+5+7+7+7+13   |
| 50 | 10 | 2+2+2+2+3+7+7+7+7+11   |
| 50 | 10 | 2+2+2+2+5+5+5+5+5+17   |
| 50 | 10 | 2+2+2+2+5+5+5+5+11+11  |
| 50 | 10 | 2+2+2+2+5+5+5+7+7+13   |
| 50 | 10 | 2+2+2+2+5+5+7+7+7+11   |
| 50 | 10 | 2+2+2+2+7+7+7+7+7+7    |
| 50 | 10 | 2+2+3+3+3+3+3+3+5+23   |
| 50 | 10 | 2+2+3+3+3+3+3+3+11+17  |
| 50 | 10 | 2+2+3+3+3+3+3+5+7+19   |
| 50 | 10 | 2+2+3+3+3+3+3+5+13+13  |
| 50 | 10 | 2+2+3+3+3+3+3+7+7+17   |
| 50 | 10 | 2+2+3+3+3+3+3+7+11+13  |

|    |    |                                               |
|----|----|-----------------------------------------------|
| 50 | 10 | 2+2+3+3+3+3+5+5+5+19                          |
| 50 | 10 | 2+2+3+3+3+3+5+5+7+17                          |
| 50 | 10 | 2+2+3+3+3+3+5+5+11+13                         |
| 50 | 10 | 2+2+3+3+3+3+5+7+11+11                         |
| 50 | 10 | 2+2+3+3+3+3+7+7+7+13                          |
| 50 | 10 | 2+2+3+3+3+5+5+5+5+17                          |
| 50 | 10 | 2+2+3+3+3+5+5+5+11+11                         |
| 50 | 10 | 2+2+3+3+3+5+5+7+7+13                          |
| 50 | 10 | 2+2+3+3+3+5+7+7+7+11                          |
| 50 | 10 | 2+2+3+3+5+5+5+5+7+13                          |
| 50 | 10 | 2+2+3+3+5+5+5+7+7+11                          |
| 50 | 10 | 2+2+3+3+5+7+7+7+7+7                           |
| 50 | 10 | 2+2+3+5+5+5+5+5+5+13                          |
| 50 | 10 | 2+2+3+5+5+5+5+5+7+11                          |
| 50 | 10 | 2+2+3+5+5+5+7+7+7+7                           |
| 50 | 10 | 2+2+5+5+5+5+5+5+5+11                          |
| 50 | 10 | 2+2+5+5+5+5+5+7+7+7                           |
| 50 | 10 | 3+3+3+3+3+3+3+3+3+23                          |
| 50 | 10 | 3+3+3+3+3+3+3+3+7+19                          |
| 50 | 10 | 3+3+3+3+3+3+3+3+13+13                         |
| 50 | 10 | 3+3+3+3+3+3+3+5+5+19                          |
| 50 | 10 | 3+3+3+3+3+3+3+5+7+17                          |
| 50 | 10 | 3+3+3+3+3+3+3+5+11+13                         |
| 50 | 10 | 3+3+3+3+3+3+3+7+11+11                         |
| 50 | 10 | 3+3+3+3+3+3+5+5+5+17                          |
| 50 | 10 | 3+3+3+3+3+3+5+5+11+11                         |
| 50 | 10 | 3+3+3+3+3+3+5+7+7+13                          |
| 50 | 10 | 3+3+3+3+3+3+7+7+7+11                          |
| 50 | 10 | 3+3+3+3+3+5+5+5+7+13                          |
| 50 | 10 | 3+3+3+3+3+5+5+7+7+11                          |
| 50 | 10 | 3+3+3+3+3+7+7+7+7+7                           |
| 50 | 10 | 3+3+3+3+5+5+5+5+5+13                          |
| 50 | 10 | 3+3+3+3+5+5+5+5+7+11                          |
| 50 | 10 | 3+3+3+3+5+5+7+7+7+7                           |
| 50 | 10 | 3+3+3+5+5+5+5+5+5+11                          |
| 50 | 10 | 3+3+3+5+5+5+5+7+7+7                           |
| 50 | 10 | 3+3+5+5+5+5+5+5+7+7                           |
| 50 | 10 | 3+5+5+5+5+5+5+5+5+7                           |
| 50 | 10 | 5+5+5+5+5+5+5+5+5+5                           |
| 50 | 25 | 2+2+2+2+2+2+2+2+2+2+2+2+2+2+2<br>+2+2+2+2+2+2 |
